# Supplementary material for: RZ Leonis Minoris Bridging between ER Ursae Majoris-Type Dwarf Nova and Novalike System
Source: arXiv:1609.08791 source file (2016-09-28)
Supplement: Supplementary file 1 [file Supplementary_draft_aph.pdf]

## E-section 1 Log of observations

The log of 2013 and 2016 observations are given in e-table 1 and ??, respectively. The key to observers and observer's information are listed in e-table 4.

## E-section 2 Supercycles in 2013 and 2016

E-figure 1 shows the general light curves of the 2013 and 2016 observations, including six supercycles and three (complete) supercycles, respectively. The period of our core observing campaign covered the 3rd (SC3) and 4th (SC4) supercycles in 2013 and the 2nd (SC2) and 3rd (SC3) supercycles in 2016. E-table 5 summarizes the characteristics of six supercycles in 2013 and three supercycles in 2016. We define that the start of a supercycle is the start of a superoutburst. Each supercycle consists of a superoutburst and usually following two normal outbursts. The exception was SC2 in 2016, when the second normal outburst following the 2nd superoutburst in 2016 was the precursor of the 3rd superoutburst. The first column of e-table 5 is the supercycle ordinal number. The 2nd and 3rd columns are JD–2456300 (2013) or JD–2457400 of the start of the supercycle, which is the start of the superoutburst, and the end of the superoutburst, respectively. The next two columns give JD of maxima of the 1st and 2nd normal outbursts. The end of the supercycle listed in the 6th column is the same as the start of the following supercycle. The last three columns give the durations (in days) of the superoutburst, the post-superoutburst phase, and the full supercycle, respectively.

E-figure 2 shows a comparison of light curves of superoutbursts, while e-figure 3 shows a comparison of light curves of non-superoutburst phases. The start and the end of each superoutburst are set to be zero for e-figure 2 and e-figure 3, respectively. As seen in e-figure 2 and in e-table 5, the superoutburst durations in 2016 were 20–48 d, which were much longer than the duration of 12–17 d in 2013. On the other hand, the typical length of non-superoutburst periods in 2016 was  $\sim 6$  d, which were shorter than that of  $\sim 9$  d in 2013.

The length of the 4th superoutburst in 2013 was much longer than those of other superoutbursts in 2013. The lengths of the following two superoutbursts were slightly shorter than those of the previous three superoutbursts while the durations of the post-superoutburst phases of the 5th and 6th supercycles were slightly longer than those of the previous three supercycles.

## E-section 3 Start of superoutbursts

Every superoutburst observed during our campaign was initiated by the 3rd outburst after the previous superoutburst, except for 2016-SO3 which was triggered by the 2nd outburst after 2016-SO2. The growth phase of superhumps (stage A), was detected during the early stage of 2013-SO4. After the initial

rise of the triggering outburst (BJD 2456380), there is was short stagnating phase. The amplitude of superhumps was very weak during this phase. Then, the object resumed rising as the amplitude of superhumps increased, and the superhumps fully grew at around the maximum of the superoutbursts. This is contrary to the expectation in Osaki, Meyer (2003) that a superoutburst of shortest orbital period SU UMa stars with the lowest mass ratio  $q$  is triggered not by the normal outburst but by the tidal instability (“case C”), as pointed out by Kato et al. (2009) for DI UMa. The observed behavior, instead, fits very well to the picture of the thermal-tidal instability (TTI) model as a “case A” superoutburst with a precursor in Osaki, Meyer (2003) as in other ordinary SU UMa-type dwarf novae (Osaki, Kato 2013a; Osaki, Kato 2013b).

## E-section 4 Period analysis

We used two methods to analyze periods of superhumps. The first is  $O - C$  analysis with times of superhump maxima determined from the light curve, and the other is analysis of the light curve with the phase dispersion minimization (PDM) method (Stellingwerf 1978) and a method using the Least Absolute Shrinkage and Selection Operator (Lasso) (Kato, Uemura 2012). The trends of outbursts were subtracted from the nightly light curves before we performed a period analysis. The  $1\sigma$  error in periods of the PDM analysis was determined by the methods in Fernie (1989), Kato et al. (2010). We used a variety of bootstrapping in estimating the robustness of the result of PDM. We analyzed 100 samples which randomly contain 50% of observations, and performed PDM analysis for these samples. The bootstrap result is shown as a form of 90% confidence intervals in the resultant  $\theta$  statistics.

The left panels of e-figures 4 and 5 show results of the PDM (red line) and Lasso (green line) analysis, respectively. The right panels of e-figure 4 and 5 show phase-averaged profiles folded by the obtained periods. Top panels are for the whole time-series dataset in flux unit, while the middle and bottom are results of the same analysis, but of the dataset during the superoutbursts and non-superoutburst phases, respectively. The second strongest peak at 0.059571(1) d in the period- $\theta$  diagram (PDM analysis) of the data during superoutbursts in 2013 is an alias of the main peak as the window function of the observations shows. The resultant periods are in agreement with the period of 0.059585(1) d derived from the PDM analysis of plateau phases of three subsequent superoutbursts in 2012 by Kato et al. (2013) and the period of 0.059542(3) d derived from the data during superoutbursts in 2016. A period analysis for datasets during the non-superoutburst phases in 2013 and 2016 gave a consistent period of 0.05970 d, though the phase-averaged data in 2016 did not show a clear hump.

E-table 1. Log of 2013 observations

| Date   | N*  | Start<br>JD–2456000 | End<br>JD–2456000 | Length<br>hr | Tel. <sup>†</sup> | Date   | N*  | Start<br>JD–2456000 | End<br>JD–2456000 | Length<br>hr | Tel. <sup>†</sup> |
|--------|-----|---------------------|-------------------|--------------|-------------------|--------|-----|---------------------|-------------------|--------------|-------------------|
| Mar 04 | 220 | 355.552234          | 355.771007        | 5.251        | 29                | Mar 30 | 343 | 381.547153          | 381.833947        | 6.883        | 7                 |
| Mar 05 | 10  | 356.864920          | 356.882300        | 0.417        | 8                 |        | 161 | 381.608210          | 381.879090        | 6.501        | 8                 |
| Mar 06 | 26  | 357.653080          | 357.717160        | 1.538        | 8                 |        | 303 | 382.132963          | 382.366863        | 5.614        | 3                 |
| Mar 07 | 84  | 358.610190          | 358.829830        | 5.271        | 8                 | Mar 31 | 59  | 382.735320          | 382.876690        | 3.393        | 8                 |
| Mar 08 | 61  | 359.666806          | 359.747106        | 1.927        | 29                |        | 174 | 383.051308          | 383.223611        | 4.135        | 1                 |
| Mar 09 | 219 | 360.551100          | 360.770880        | 5.275        | 29                |        | 197 | 383.400900          | 383.558920        | 3.792        | 5                 |
|        | 25  | 360.620470          | 360.675170        | 1.313        | 6                 | Apr 01 | 129 | 383.608030          | 383.786240        | 4.277        | 8                 |
| Mar 11 | 91  | 362.543440          | 362.750820        | 4.977        | 6                 |        | 41  | 384.127604          | 384.172002        | 1.066        | 1                 |
|        | 19  | 362.728520          | 362.748400        | 0.477        | 8                 |        | 220 | 384.404410          | 384.573780        | 4.065        | 5                 |
|        | 158 | 363.063125          | 363.291782        | 5.488        | 1                 | Apr 02 | 201 | 384.540320          | 384.749590        | 5.022        | 6                 |
| Mar 12 | 71  | 363.726590          | 363.884850        | 3.798        | 8                 |        | 328 | 384.553507          | 384.825220        | 6.521        | 7                 |
|        | 38  | 363.728530          | 363.803390        | 1.774        | 8                 |        | 119 | 385.339560          | 385.439200        | 2.391        | RJWB              |
|        | 64  | 364.074456          | 364.178368        | 2.494        | 1                 |        | 243 | 385.401620          | 385.584870        | 4.398        | 5                 |
| Mar 13 | 133 | 364.582870          | 364.762330        | 4.307        | 8                 | Apr 03 | 349 | 385.544896          | 385.831435        | 6.877        | 7                 |
| Mar 14 | 244 | 365.539700          | 365.750150        | 5.051        | 6                 |        | 157 | 386.036655          | 386.242674        | 4.944        | 1                 |
|        | 211 | 365.557211          | 365.770926        | 5.129        | 29                |        | 265 | 386.394350          | 386.601480        | 4.971        | 5                 |
|        | 85  | 365.791560          | 365.886600        | 2.281        | 8                 | Apr 04 | 318 | 386.577222          | 386.851759        | 6.589        | 7                 |
|        | 146 | 366.123970          | 366.301551        | 4.262        | 1                 |        | 142 | 386.756480          | 386.866300        | 2.636        | 8                 |
| Mar 15 | 244 | 366.539940          | 366.750410        | 5.051        | 6                 |        | 148 | 387.051493          | 387.214931        | 3.923        | 1                 |
|        | 187 | 366.593090          | 366.909050        | 7.583        | 8                 |        | 299 | 387.121262          | 387.416713        | 7.091        | 3                 |
|        | 89  | 366.830822          | 366.886493        | 1.336        | 9                 |        | 110 | 387.343800          | 387.438960        | 2.284        | RJWB              |
|        | 157 | 367.088403          | 367.262396        | 4.176        | 1                 |        | 247 | 387.396100          | 387.587560        | 4.595        | 5                 |
|        | 127 | 367.088414          | 367.207581        | 2.860        | 2b                | Apr 05 | 262 | 387.562700          | 387.780600        | 5.230        | 7                 |
|        | 233 | 367.105250          | 367.323380        | 5.235        | 3                 |        | 260 | 388.141528          | 388.344676        | 4.876        | 3                 |
| Mar 16 | 90  | 367.854965          | 367.910486        | 1.333        | 9                 |        | 157 | 388.409110          | 388.537270        | 3.076        | 5                 |
|        | 133 | 368.074352          | 368.220648        | 3.511        | 1                 | Apr 06 | 461 | 389.114456          | 389.410278        | 7.100        | 3                 |
|        | 130 | 368.095243          | 368.209352        | 2.792        | 2b                |        | 134 | 389.330710          | 389.436170        | 2.531        | RJWB              |
|        | 272 | 368.247510          | 368.452130        | 4.911        | 3                 |        | 82  | 389.410060          | 389.474120        | 1.537        | 5                 |
|        | 96  | 368.367930          | 368.447250        | 1.904        | 5                 | Apr 07 | 86  | 389.629180          | 389.729630        | 2.411        | 8                 |
| Mar 17 | 90  | 368.851285          | 368.906944        | 1.336        | 9                 |        | 223 | 389.970058          | 390.160694        | 4.575        | 2a                |
|        | 11  | 369.095694          | 369.104479        | 0.211        | 2b                |        | 92  | 390.129433          | 390.209699        | 1.926        | 2b                |
|        | 315 | 369.126080          | 369.402430        | 6.632        | 3                 |        | 196 | 390.190278          | 390.314965        | 2.992        | 3                 |
| Mar 18 | 90  | 369.742350          | 369.798090        | 1.338        | 9                 | Apr 08 | 169 | 390.620930          | 390.817640        | 4.721        | 8                 |
|        | 65  | 370.157847          | 370.214317        | 1.355        | 2b                |        | 143 | 390.969595          | 391.079664        | 2.642        | 1                 |
|        | 132 | 370.434590          | 370.580720        | 3.507        | 5                 |        | 181 | 391.351790          | 391.561270        | 5.028        | 4                 |
| Mar 19 | 43  | 370.739456          | 370.792789        | 1.280        | 9                 | Apr 09 | 182 | 391.540270          | 391.728880        | 4.527        | 6                 |
|        | 130 | 371.330540          | 371.436690        | 2.548        | 3                 |        | 120 | 391.628780          | 391.773940        | 3.484        | 8                 |
| Mar 20 | 519 | 371.526215          | 371.792905        | 6.401        | 7                 |        | 294 | 392.184826          | 392.388843        | 4.896        | 3                 |
|        | 207 | 371.602176          | 371.812639        | 5.051        | 29                | Apr 10 | 178 | 392.549990          | 392.758370        | 5.001        | 6                 |
|        | 77  | 371.723403          | 371.779653        | 1.350        | 9                 |        | 133 | 393.357850          | 393.531820        | 4.175        | 4                 |
|        | 89  | 371.747770          | 371.883000        | 3.246        | 8                 | Apr 11 | 101 | 394.032512          | 394.156389        | 2.973        | 1                 |
|        | 69  | 372.136180          | 372.191120        | 1.319        | 3                 |        | 282 | 394.188113          | 394.396574        | 5.003        | 3                 |
| Mar 21 | 231 | 372.573785          | 372.749398        | 4.215        | 7                 | Apr 12 | 45  | 395.388320          | 395.422590        | 0.822        | 5                 |
|        | 32  | 372.627180          | 372.720310        | 2.235        | 8                 | Apr 13 | 148 | 395.658611          | 395.768287        | 2.632        | 9                 |
|        | 162 | 372.654178          | 372.812326        | 3.796        | 29                |        | 220 | 395.936794          | 396.104144        | 4.016        | 1                 |
|        | 131 | 373.049977          | 373.194155        | 3.460        | 1                 | Apr 14 | 111 | 396.622870          | 396.778810        | 3.743        | 8                 |
|        | 78  | 373.214525          | 373.282500        | 1.631        | 2b                |        | 180 | 396.658646          | 396.767986        | 2.624        | 9                 |
| Mar 22 | 412 | 373.554988          | 373.839664        | 6.832        | 7                 |        | 73  | 397.156181          | 397.219699        | 1.524        | 2b                |
|        | 246 | 373.566400          | 373.812917        | 5.916        | 29                | Apr 15 | 70  | 397.643190          | 397.788700        | 3.492        | 8                 |
|        | 239 | 373.970116          | 374.166991        | 4.725        | 2a                |        | 13  | 397.966424          | 398.006285        | 0.957        | 1                 |
|        | 75  | 374.154398          | 374.227662        | 1.758        | 2b                | Apr 16 | 49  | 398.552440          | 398.634100        | 1.960        | 6                 |
|        | 50  | 374.237510          | 374.277210        | 0.953        | 3                 | Apr 17 | 55  | 399.734980          | 399.810580        | 1.814        | 8                 |
| Mar 23 | 201 | 374.530995          | 374.710567        | 4.310        | 7                 |        | 205 | 399.961319          | 400.193657        | 5.576        | 1                 |
|        | 91  | 374.690200          | 374.888890        | 4.769        | 8                 |        | 114 | 400.428260          | 400.526610        | 2.360        | 5                 |
| Mar 24 | 125 | 375.626810          | 375.883130        | 6.152        | 8                 | Apr 19 | 59  | 401.961181          | 402.088669        | 3.060        | 1                 |
| Mar 25 | 107 | 376.608830          | 376.882260        | 6.562        | 8                 |        | 154 | 402.377880          | 402.504540        | 3.040        | 5                 |
|        | 139 | 377.088669          | 377.277130        | 4.523        | 1                 | Apr 22 | 90  | 405.135208          | 405.213704        | 1.884        | 2b                |
| Mar 26 | 147 | 377.608020          | 377.823030        | 5.160        | 8                 | Apr 23 | 63  | 405.640340          | 405.715460        | 1.803        | 8                 |
| Mar 27 | 137 | 378.608130          | 378.867300        | 6.220        | 8                 |        | 110 | 406.108368          | 406.204398        | 2.305        | 2b                |
| Mar 28 | 314 | 379.564120          | 379.830914        | 6.403        | 7                 | Apr 24 | 136 | 407.091308          | 407.210185        | 2.853        | 2b                |
|        | 97  | 379.602523          | 379.708275        | 2.538        | 29                | Apr 25 | 246 | 407.573819          | 407.789433        | 5.175        | 7                 |
| Mar 29 | 85  | 380.573785          | 380.667708        | 2.254        | 29                | Apr 26 | 31  | 408.987315          | 409.054988        | 1.624        | 1                 |
|        | 116 | 380.638370          | 380.825390        | 4.488        | 8                 | Apr 27 | 176 | 409.557270          | 409.708080        | 3.619        | 6                 |
|        | 133 | 381.120579          | 381.305637        | 4.441        | 3                 | Apr 28 | 175 | 410.947847          | 411.121157        | 4.159        | 1                 |
|        | 75  | 381.405540          | 381.462890        | 1.376        | 5                 | Apr 29 | 150 | 411.988912          | 412.120741        | 3.164        | 2b                |

\*Number of observations.

† see e-table 4

E-table 2. Log of 2016 observations

| Date   | N*  | Start<br>JD−2457000 | End<br>JD−2457000 | Length<br>hr | Tel. <sup>†</sup> | Date   | N*  | Start<br>JD−2457000 | End<br>JD−2457000 | Length<br>hr | Tel. <sup>†</sup> |
|--------|-----|---------------------|-------------------|--------------|-------------------|--------|-----|---------------------|-------------------|--------------|-------------------|
| Feb 25 | 140 | 443.5857            | 443.6995          | 2.731        | 10                | Mar 27 | 4   | 475.3336            | 475.3363          | 0.065        | 10                |
| Feb 26 | 308 | 444.5406            | 444.7725          | 5.566        | 6                 |        | 111 | 475.3572            | 475.4836          | 3.034        | 11a               |
| Feb 27 | 88  | 445.5877            | 445.6820          | 2.263        | 11a               | Mar 28 | 11  | 475.7379            | 475.7556          | 0.425        | 26                |
|        | 163 | 446.2101            | 446.3469          | 3.283        | 15                |        | 161 | 475.9423            | 476.1721          | 5.515        | 14                |
|        | 6   | 446.4863            | 446.6622          | 4.222        | 10                |        | 269 | 476.0427            | 476.1418          | 2.378        | 17                |
| Feb 28 | 52  | 447.0112            | 447.1183          | 2.570        | 14                |        | 344 | 476.0625            | 476.1920          | 3.108        | 1                 |
|        | 34  | 447.4024            | 447.4287          | 0.631        | 10                |        | 133 | 476.3265            | 476.5156          | 4.538        | 11ab              |
| Feb 29 | 125 | 447.9509            | 448.2128          | 6.286        | 14                |        | 9   | 476.3497            | 476.5714          | 5.321        | 10                |
|        | 10  | 448.3061            | 448.6080          | 7.246        | 10                |        | 13  | 476.4380            | 476.4553          | 0.415        | 13a               |
|        | 100 | 448.3495            | 448.5151          | 3.974        | 13a               | Mar 29 | 258 | 476.5523            | 476.6782          | 3.022        | CDK               |
| Mar 01 | 9   | 448.9763            | 448.9952          | 0.454        | 14                |        | 250 | 476.5748            | 476.7502          | 4.210        | BJA               |
|        | 5   | 449.3077            | 449.6009          | 7.037        | 10                |        | 358 | 476.6484            | 476.9582          | 7.435        | JJI               |
|        | 55  | 449.4812            | 449.5587          | 1.860        | 13a               |        | 50  | 476.6705            | 476.7401          | 1.670        | 26                |
| Mar 02 | 9   | 450.3155            | 450.5017          | 4.469        | 10                |        | 11  | 477.2263            | 477.2481          | 0.523        | 13b               |
| Mar 03 | 10  | 451.3084            | 451.5800          | 6.518        | 10                |        | 331 | 477.3728            | 477.5454          | 4.142        | 11a               |
| Mar 04 | 6   | 452.3287            | 452.6008          | 6.530        | 10                |        | 51  | 477.4256            | 477.4974          | 1.723        | 13a               |
|        | 108 | 452.4936            | 452.6082          | 2.750        | 11b               | Mar 30 | 171 | 477.5133            | 477.7904          | 6.650        | MZK               |
| Mar 05 | 10  | 453.2227            | 453.2346          | 0.286        | 13c               |        | 143 | 477.5396            | 477.6471          | 2.580        | CDK               |
|        | 9   | 453.2230            | 453.2336          | 0.254        | 13c               |        | 449 | 477.6467            | 477.9581          | 7.474        | JJI               |
|        | 8   | 453.2233            | 453.2339          | 0.254        | 13c               |        | 406 | 478.0063            | 478.2161          | 5.035        | 15                |
|        | 3   | 453.3284            | 453.3297          | 0.031        | 10                |        | 136 | 478.0119            | 478.0949          | 1.992        | 18                |
| Mar 06 | 54  | 454.2038            | 454.3019          | 2.354        | 13c               |        | 9   | 478.0967            | 478.1248          | 0.674        | 1                 |
|        | 3   | 454.3259            | 454.3272          | 0.031        | 10                |        | 305 | 478.3621            | 478.5464          | 4.423        | 23                |
|        | 67  | 454.3420            | 454.4382          | 2.309        | 13a               |        | 48  | 478.3739            | 478.4740          | 2.402        | 13a               |
| Mar 07 | 260 | 455.0242            | 455.2480          | 5.371        | 16                |        | 93  | 478.4031            | 478.5035          | 2.410        | 20                |
|        | 74  | 455.2168            | 455.3316          | 2.755        | 13a               | Mar 31 | 357 | 478.6474            | 478.9584          | 7.464        | JJI               |
|        | 3   | 455.3218            | 455.3231          | 0.031        | 10                |        | 52  | 478.7555            | 478.8347          | 1.901        | 26                |
| Mar 08 | 86  | 455.5136            | 455.5838          | 1.685        | RAE               |        | 86  | 479.2679            | 479.3287          | 1.459        | 19                |
|        | 192 | 456.2492            | 456.5365          | 6.895        | 13b               |        | 206 | 479.3408            | 479.5856          | 5.875        | 10                |
|        | 236 | 456.2894            | 456.5975          | 7.394        | 19                |        | 203 | 479.3410            | 479.5118          | 4.099        | 11a               |
|        | 3   | 456.3259            | 456.3275          | 0.038        | 10                |        | 101 | 479.3414            | 479.5550          | 5.126        | 13a               |
| Mar 09 | 122 | 457.2200            | 457.3999          | 4.318        | 13b               |        | 119 | 479.3883            | 479.4786          | 2.167        | 22                |
|        | 140 | 457.3675            | 457.5683          | 4.819        | 13a               | Apr 01 | 38  | 479.5035            | 479.5313          | 0.667        | JSJ               |
| Mar 10 | 102 | 457.5287            | 457.6062          | 1.860        | 5                 |        | 207 | 479.5750            | 479.7989          | 5.374        | 6                 |
|        | 41  | 458.2058            | 458.2653          | 1.428        | 13b               |        | 331 | 479.6604            | 479.9483          | 6.910        | JJI               |
|        | 3   | 458.3293            | 458.3305          | 0.029        | 10                |        | 88  | 480.0547            | 480.2378          | 4.394        | 14                |
|        | 140 | 458.3626            | 458.4685          | 2.542        | 5                 |        | 76  | 480.1715            | 480.2264          | 1.318        | 1                 |
|        | 242 | 458.4537            | 458.6308          | 4.250        | 20                |        | 154 | 480.2715            | 480.4907          | 5.261        | 11b               |
| Mar 11 | 152 | 459.0435            | 459.1662          | 2.945        | 16                |        | 119 | 480.3410            | 480.4313          | 2.167        | 22                |
|        | 3   | 459.3239            | 459.3252          | 0.031        | 10                |        | 25  | 480.3879            | 480.4200          | 0.770        | 13c               |
| Mar 13 | 3   | 460.5833            | 460.5845          | 0.029        | 10                | Apr 02 | 240 | 480.5654            | 480.7540          | 4.526        | 6                 |
|        | 44  | 461.2710            | 461.3843          | 2.719        | 13b               |        | 205 | 480.6581            | 480.8437          | 4.454        | JJI               |
|        | 3   | 461.3193            | 461.3208          | 0.036        | 10                |        | 100 | 480.7188            | 480.8658          | 3.528        | 26                |
|        | 266 | 461.3260            | 461.5176          | 4.598        | 20                |        | 142 | 480.9808            | 481.0870          | 2.549        | 1                 |
|        | 163 | 461.3356            | 461.4600          | 2.986        | 5                 |        | 46  | 481.0118            | 481.1569          | 3.482        | 14                |
|        | 63  | 461.3359            | 461.4263          | 2.170        | 13a               |        | 74  | 481.2966            | 481.4262          | 3.110        | 13c               |
| Mar 14 | 223 | 462.3293            | 462.4898          | 3.852        | 20                |        | 22  | 481.4266            | 481.4879          | 1.471        | 19                |
|        | 3   | 462.3594            | 462.3609          | 0.036        | 10                | Apr 03 | 22  | 481.6034            | 481.6851          | 1.961        | 24                |
| Mar 15 | 83  | 463.2302            | 463.3276          | 2.338        | 13b               |        | 203 | 481.6509            | 481.9427          | 7.003        | JJI               |
|        | 184 | 463.3151            | 463.5794          | 6.343        | 13a               |        | 99  | 481.7390            | 481.8941          | 3.722        | 26                |
| Mar 16 | 210 | 464.2248            | 464.4858          | 6.264        | 13b               |        | 50  | 482.2303            | 482.3347          | 2.506        | 13a               |
|        | 48  | 464.2485            | 464.3981          | 3.590        | 13a               |        | 44  | 482.2776            | 482.3244          | 1.123        | 19                |
|        | 279 | 464.2714            | 464.4942          | 5.347        | 21                |        | 82  | 482.3054            | 482.5122          | 4.963        | 11b               |
|        | 3   | 464.3230            | 464.3245          | 0.036        | 10                | Apr 04 | 121 | 482.5533            | 482.7539          | 4.814        | CDK               |
| Mar 17 | 276 | 465.2772            | 465.4953          | 5.234        | 21                |        | 240 | 482.6256            | 482.8379          | 5.095        | 27                |
|        | 276 | 465.3077            | 465.5202          | 5.100        | 20                |        | 93  | 482.7722            | 482.9188          | 3.518        | 26                |
| Mar 19 | 247 | 467.2907            | 467.4856          | 4.678        | 21                |        | 5   | 483.0042            | 483.0349          | 0.737        | 14                |
|        | 3   | 467.3370            | 467.3385          | 0.036        | 10                |        | 112 | 483.2380            | 483.4809          | 5.830        | 13a               |
| Mar 20 | 175 | 468.3940            | 468.5291          | 3.242        | 20                |        | 175 | 483.3188            | 483.5431          | 5.383        | 19                |
| Mar 22 | 167 | 470.0461            | 470.1199          | 1.771        | 18                | Apr 05 | 23  | 483.6019            | 483.6833          | 1.954        | 24                |
|        | 17  | 470.4136            | 470.4811          | 1.620        | 11b               |        | 56  | 483.7693            | 483.8523          | 1.992        | 26                |
| Mar 24 | 154 | 471.6751            | 471.9091          | 5.616        | 26                |        | 623 | 483.9559            | 484.2356          | 6.713        | 17                |
|        | 148 | 471.9612            | 472.1645          | 4.879        | 14                |        | 289 | 484.0070            | 484.1154          | 2.602        | 1                 |
|        | 341 | 472.0644            | 472.2142          | 3.595        | 18                |        | 138 | 484.1009            | 484.1624          | 1.476        | 18                |
|        | 236 | 472.2933            | 472.5542          | 6.262        | 11a               |        | 82  | 484.2882            | 484.3727          | 2.028        | 11ab              |
|        | 49  | 472.3260            | 472.3925          | 1.596        | 19                |        | 302 | 484.2899            | 484.5458          | 6.142        | 19                |
|        | 6   | 472.3322            | 472.3359          | 0.089        | 10                |        | 285 | 484.3340            | 484.5556          | 5.318        | 21                |
| Mar 25 | 799 | 472.9369            | 473.2369          | 7.200        | 17                |        | 162 | 484.3397            | 484.4640          | 2.983        | 20                |
|        | 170 | 472.9386            | 473.1800          | 5.794        | 14                |        | 68  | 484.3406            | 484.4955          | 3.718        | 13a               |
|        | 94  | 473.3175            | 473.4769          | 3.826        | BSM               |        | 92  | 484.3412            | 484.4224          | 1.949        | 22                |
|        | 175 | 473.3306            | 473.6047          | 6.578        | 10                |        | 284 | 484.3419            | 484.5563          | 5.146        | 10                |
|        | 119 | 473.3972            | 473.4876          | 2.170        | 22                |        | 143 | 484.4916            | 484.6036          | 2.688        | 25                |
| Mar 26 | 77  | 473.7326            | 473.8967          | 3.938        | 26                | Apr 06 | 86  | 484.6453            | 484.7304          | 2.042        | 27                |
|        | 167 | 473.9363            | 474.1759          | 5.750        | 14                |        | 70  | 484.7944            | 484.8538          | 1.426        | JJI               |
|        | 82  | 473.9651            | 474.0061          | 0.984        | 18                |        | 50  | 484.8077            | 484.8784          | 1.697        | 26                |
|        | 402 | 474.0114            | 474.1619          | 3.612        | 1                 |        | 302 | 485.2275            | 485.4660          | 5.724        | 13b               |
| Mar 27 | 80  | 474.6436            | 474.7825          | 3.334        | MZK               |        | 81  | 485.2499            | 485.5557          | 7.339        | 13a               |
|        | 122 | 474.9779            | 475.1742          | 4.711        | 14                |        | 349 | 485.3339            | 485.5516          | 5.225        | 10                |
|        | 168 | 475.0347            | 475.1881          | 3.682        | 16                | Apr 07 | 142 | 485.5148            | 485.6264          | 2.678        | 25                |
|        | 6   | 475.1037            | 475.1112          | 0.180        | 1                 |        | 23  | 485.6031            | 485.6876          | 2.028        | 24                |
|        | 45  | 475.2998            | 475.3845          | 2.033        | 13a               |        | 100 | 485.6481            | 485.8015          | 3.682        | 26                |

\* Number of observations.

† see e-table 4

E-table 3. Log of 2016 observations (continued)

| Date   | N** | Start<br>JD–2457000 | End<br>JD–2457000 | Length<br>hr | Tel. <sup>†</sup> | Date   | N*  | Start<br>JD–2457000 | End<br>JD–2457000 | Length<br>hr | Tel. <sup>††</sup> |
|--------|-----|---------------------|-------------------|--------------|-------------------|--------|-----|---------------------|-------------------|--------------|--------------------|
| Apr 07 | 218 | 485.6568            | 485.8538          | 4.728        | JJI               | Apr 29 | 79  | 508.3715            | 508.4326          | 1.466        | 5                  |
|        | 107 | 485.9822            | 486.2369          | 6.113        | 14                | Apr 30 | 6   | 508.5500            | 508.5538          | 0.091        | JSJ                |
|        | 365 | 486.2351            | 486.5288          | 7.049        | 13b               |        | 382 | 508.9389            | 509.1710          | 5.570        | 15                 |
|        | 92  | 486.3111            | 486.5314          | 5.287        | 11a               |        | 78  | 508.9552            | 509.1414          | 4.469        | 14                 |
|        | 159 | 486.4015            | 486.4906          | 2.138        | 10                |        | 104 | 509.3828            | 509.4663          | 2.004        | 5                  |
| Apr 08 | 200 | 486.6284            | 486.8148          | 4.474        | 27                | May 01 | 69  | 510.0183            | 510.1653          | 3.528        | 14                 |
|        | 231 | 486.6552            | 486.8544          | 4.781        | JJI               |        | 80  | 510.2731            | 510.4452          | 4.130        | 13b                |
|        | 48  | 486.7576            | 486.8347          | 1.850        | 26                | May 02 | 72  | 510.9627            | 511.1188          | 3.746        | 14                 |
|        | 117 | 486.9494            | 487.1212          | 4.123        | 14                |        | 39  | 511.2749            | 511.3664          | 2.196        | 13b                |
|        | 355 | 486.9822            | 487.1151          | 3.190        | 1                 |        | 98  | 511.3784            | 511.4506          | 1.733        | 5                  |
|        | 404 | 486.9987            | 487.1640          | 3.967        | 17                |        | 88  | 511.3797            | 511.4440          | 1.543        | 20                 |
|        | 225 | 487.3365            | 487.4838          | 3.535        | 10                |        | 14  | 511.4074            | 511.4172          | 0.235        | JSJ                |
|        | 139 | 487.4916            | 487.6036          | 2.688        | 25                | May 03 | 107 | 512.3907            | 512.4704          | 1.913        | 5                  |
| Apr 09 | 200 | 487.6295            | 487.8108          | 4.351        | 27                | May 04 | 252 | 512.9712            | 513.0803          | 2.618        | 18                 |
|        | 82  | 487.9824            | 488.1787          | 4.711        | 14                |        | 72  | 512.9781            | 513.1276          | 3.588        | 14                 |
|        | 144 | 488.0105            | 488.0642          | 1.289        | 1                 | May 05 | 192 | 513.9424            | 514.0745          | 3.170        | 15                 |
|        | 192 | 488.3428            | 488.4631          | 2.887        | 10                |        | 277 | 514.3279            | 514.4201          | 2.213        | 13c                |
|        | 278 | 488.3449            | 488.5450          | 4.802        | 20                |        | 120 | 514.3912            | 514.5294          | 3.317        | 5                  |
|        | 180 | 488.4304            | 488.5344          | 2.496        | 28                | May 07 | 19  | 515.9760            | 516.0664          | 2.170        | 14                 |
| Apr 10 | 153 | 488.9487            | 489.0954          | 3.521        | 15                |        | 70  | 516.0351            | 516.0982          | 1.514        | 15                 |
|        | 210 | 489.0329            | 489.1267          | 2.251        | 17                |        | 150 | 516.2687            | 516.4381          | 4.066        | 13b                |
|        | 109 | 489.2802            | 489.3552          | 1.800        | 12                |        | 73  | 516.3726            | 516.4261          | 1.284        | 20                 |
|        | 163 | 489.3331            | 489.4576          | 2.988        | 22                | May 08 | 18  | 517.4481            | 517.4624          | 0.343        | JSJ                |
| Apr 11 | 200 | 489.6443            | 489.8301          | 4.459        | 27                | May 09 | 75  | 518.2714            | 518.3832          | 2.683        | 13b                |
|        | 114 | 489.9405            | 490.2078          | 6.415        | 14                |        | 64  | 518.3812            | 518.4317          | 1.212        | 21                 |
|        | 373 | 489.9834            | 490.1230          | 3.350        | 1                 | May 11 | 56  | 520.0079            | 520.1245          | 2.798        | 14                 |
|        | 598 | 490.0021            | 490.2471          | 5.880        | 17                |        | 234 | 520.0207            | 520.1205          | 2.395        | 17                 |
|        | 205 | 490.3252            | 490.5019          | 4.241        | 13b               |        | 174 | 520.3169            | 520.4513          | 3.226        | 21                 |
| Apr 12 | 120 | 490.3395            | 490.4254          | 2.062        | 19                |        | 66  | 520.3959            | 520.4713          | 1.810        | 11a                |
|        | 149 | 490.5845            | 490.6875          | 2.472        | BJA               | May 12 | 68  | 520.9566            | 521.0998          | 3.437        | 14                 |
|        | 23  | 490.6056            | 490.6901          | 2.028        | 24                |        | 146 | 520.9864            | 521.0683          | 1.966        | 18                 |
|        | 250 | 490.6332            | 490.8595          | 5.431        | 27                |        | 210 | 521.0410            | 521.1805          | 3.348        | 15                 |
|        | 72  | 491.0189            | 491.1832          | 3.943        | 14                |        | 123 | 521.3974            | 521.4858          | 2.122        | 20                 |
| Apr 13 | 98  | 491.3889            | 491.4679          | 1.896        | 5                 |        | 126 | 521.4081            | 521.5087          | 2.414        | 5                  |
|        | 339 | 491.5531            | 491.7303          | 4.253        | MZK               | May 13 | 48  | 521.9715            | 522.0705          | 2.376        | 14                 |
|        | 62  | 492.3977            | 492.4689          | 1.709        | 13b               |        | 35  | 522.3469            | 522.3957          | 1.171        | 13a                |
|        | 74  | 492.4013            | 492.5067          | 2.530        | 13a               | May 14 | 8   | 522.9841            | 523.0051          | 0.504        | 14                 |
| Apr 14 | 150 | 492.5844            | 492.6880          | 2.486        | BJA               |        | 15  | 523.2771            | 523.3102          | 0.794        | 13b                |
|        | 36  | 492.6859            | 492.7551          | 1.661        | 26                | May 15 | 207 | 523.9575            | 524.0464          | 2.134        | 18                 |
|        | 116 | 492.9541            | 493.1972          | 5.834        | 14                |        | 40  | 524.3231            | 524.3842          | 1.466        | 13b                |
|        | 286 | 493.0071            | 493.1144          | 2.575        | 1                 |        | 81  | 524.3898            | 524.4570          | 1.613        | 20                 |
| Apr 15 | 319 | 493.5189            | 493.6882          | 4.063        | MZK               | May 16 | 79  | 525.3944            | 525.4585          | 1.538        | 5                  |
|        | 100 | 493.6835            | 493.8217          | 3.317        | 26                |        | 89  | 525.4008            | 525.4651          | 1.543        | 20                 |
|        | 455 | 493.9797            | 494.1501          | 4.090        | 1                 | May 17 | 51  | 525.9557            | 526.0677          | 2.688        | 14                 |
|        | 344 | 494.0478            | 494.2151          | 4.015        | 15                | May 18 | 61  | 526.9565            | 527.0827          | 3.029        | 14                 |
| Apr 16 | 31  | 494.0754            | 494.1386          | 1.517        | 14                |        | 164 | 526.9752            | 527.0456          | 1.690        | 18                 |
|        | 384 | 494.5204            | 494.7216          | 4.829        | MZK               |        | 165 | 527.0281            | 527.1255          | 2.338        | 15                 |
|        | 144 | 495.2468            | 495.4620          | 5.165        | 13b               | May 19 | 109 | 527.4102            | 527.4966          | 2.074        | 5                  |
|        | 217 | 495.3649            | 495.5275          | 3.902        | 20                |        | 93  | 528.2761            | 528.4127          | 3.278        | 13b                |
| Apr 17 | 261 | 495.5421            | 495.7255          | 4.402        | MZK               |        | 155 | 528.3083            | 528.4296          | 2.911        | 21                 |
|        | 196 | 495.6414            | 495.8324          | 4.584        | 27                | May 20 | 83  | 529.2658            | 529.3905          | 2.993        | 13b                |
|        | 59  | 495.9408            | 496.0629          | 2.930        | 14                |        | 88  | 529.2774            | 529.4045          | 3.050        | 13a                |
|        | 189 | 495.9497            | 496.0382          | 2.124        | 15                |        | 145 | 529.3196            | 529.4345          | 2.758        | 21                 |
|        | 174 | 495.9811            | 496.0489          | 1.627        | 17                |        | 37  | 529.3804            | 529.4552          | 1.795        | 11a                |
|        | 56  | 496.2940            | 496.4138          | 2.875        | 13b               | May 22 | 205 | 530.9446            | 531.0836          | 3.336        | 15                 |
|        | 276 | 496.3547            | 496.5600          | 4.927        | 20                |        | 73  | 531.2843            | 531.3934          | 2.618        | 13a                |
|        | 149 | 496.3649            | 496.4767          | 2.683        | 5                 |        | 71  | 531.3128            | 531.4647          | 3.646        | 11a                |
| Apr 18 | 65  | 497.3046            | 497.4506          | 3.504        | 13b               |        | 59  | 531.3999            | 531.4425          | 1.022        | 20                 |
| Apr 19 | 10  | 497.9370            | 497.9560          | 0.456        | 14                |        | 81  | 531.4083            | 531.4837          | 1.810        | 5                  |
|        | 453 | 497.9484            | 498.1201          | 4.121        | 17                | May 23 | 51  | 532.0432            | 532.0982          | 1.320        | 17                 |
|        | 480 | 497.9864            | 498.1662          | 4.315        | 1                 |        | 59  | 532.3266            | 532.4118          | 2.045        | 21                 |
|        | 165 | 498.3400            | 498.4645          | 2.988        | 22                |        | 77  | 532.3401            | 532.4595          | 2.866        | 11a                |
|        | 100 | 498.3739            | 498.4452          | 1.711        | 19                |        | 45  | 532.4078            | 532.4852          | 1.858        | 5                  |
| Apr 20 | 305 | 498.5225            | 498.7481          | 5.414        | MZK               | May 24 | 62  | 533.3491            | 533.4460          | 2.326        | 21                 |
|        | 224 | 498.6457            | 498.8387          | 4.632        | 27                |        | 45  | 533.4151            | 533.4653          | 1.205        | 5                  |
|        | 60  | 499.4259            | 499.4747          | 1.171        | RAE               | May 25 | 60  | 534.3162            | 534.3827          | 1.596        | 11a                |
| Apr 21 | 269 | 499.5196            | 499.7106          | 4.584        | MZK               | May 26 | 48  | 535.3201            | 535.4116          | 2.196        | 11a                |
|        | 249 | 499.6416            | 499.8574          | 5.179        | 27                | May 28 | 143 | 536.9606            | 537.0845          | 2.974        | 15                 |
|        | 100 | 499.6932            | 499.8281          | 3.238        | 26                |        | 89  | 537.3397            | 537.4086          | 1.654        | 21                 |
|        | 61  | 500.2495            | 500.3516          | 2.450        | 13a               | May 29 | 6   | 538.4142            | 538.4186          | 0.106        | 20                 |
| Apr 22 | 199 | 500.9451            | 501.0445          | 2.386        | 17                | May 30 | 48  | 539.4317            | 539.4874          | 1.337        | 5                  |
|        | 119 | 501.2556            | 501.4363          | 4.337        | 13a               | Jun 01 | 49  | 541.0728            | 541.1096          | 0.883        | 15                 |
| Apr 23 | 91  | 502.3646            | 502.4304          | 1.579        | 20                |        | 31  | 541.2937            | 541.3641          | 1.690        | 13b                |
| Apr 24 | 262 | 502.5218            | 502.7061          | 4.423        | MZK               | Jun 02 | 92  | 541.9742            | 542.0698          | 2.294        | 17                 |
|        | 25  | 503.2818            | 503.3163          | 0.828        | 13a               |        | 79  | 542.4136            | 542.4740          | 1.450        | 5                  |
|        | 172 | 503.3523            | 503.4784          | 3.026        | 10                |        | 14  | 542.4280            | 542.4382          | 0.245        | 20                 |
| Apr 27 | 96  | 506.3969            | 506.4655          | 1.646        | 20                | Jun 03 | 41  | 543.3876            | 543.4374          | 1.195        | 11b                |
| Apr 28 | 78  | 507.2639            | 507.4317          | 4.027        | 13b               |        | 81  | 543.4186            | 543.4789          | 1.447        | 5                  |
| Apr 29 | 103 | 507.9438            | 508.1583          | 5.148        | 14                | Jun 05 | 113 | 544.9479            | 545.0250          | 1.850        | 15                 |
|        | 325 | 507.9570            | 508.1023          | 3.487        | 18                | Jun 10 | 124 | 549.9734            | 550.0211          | 1.145        | 17                 |
|        | 338 | 508.0310            | 508.2001          | 4.058        | 15                |        |     |                     |                   |              |                    |

\* Number of observations.

<sup>†</sup> see e-table 4

**E-table 4.** List of sites and instruments

| No.* | Obscaroty (or site)    | Coordinate           | Telescope  | Camera            | Filter  | Software          |
|------|------------------------|----------------------|------------|-------------------|---------|-------------------|
| 1    | Osaka Kyoiku Univ.     | 135:39:00E 34:33:06N | 51-cm      | Andor DW436       | V,clear | IRAF              |
| 2a   | Lulin Obs.             | 120:52:25E 23:28:07N | 1.0-m      | PI 1300B          | B,V,R   | SExtractor        |
| 2b   | Lulin Obs.             | 120:52:25E 23:28:07N | 40-cm      | Apogee Alta U42   | V,none  | SExtractor        |
| 3    | Tien Shan Obs.         | 76:58:16E 43:03:27N  | 1.0-m      | Apogee Alta F9000 | B,V,R,L | MaxIm DL          |
| 4    | Hankasalmi Obs.        | 26:35:47E 62:15:17N  | 40-cm      | SBIG STL-1001E    | V       | VBScript          |
| 5    | Furzehill Obs.         | 04:05:50W 51:35:49N  | 35-cm      | SXVR-H16          | C       | AIP4Win           |
| 6    | Rolling Hills Obs.     | 81:43:27W 28:33:27N  | 25-cm      | SBIG ST-9XE       | V,clear |                   |
| 7    | DeKalb Obs.            | 85:04:22W 41:18:38N  | 41-cm      | SBIG ST10XME      | V,clear | AIP4Win           |
| 8    | T5 New Mexico          | 105:31W 32:54N       | 25-cm      | SBIG ST10XME      | V,clear | VPhot             |
| 9    | Tenagra Obs.           | 110:52:45W 31:27:44N | 81-cm      | Apogee Alta F6    | B,V,R   | SExtractor        |
| 10   | Obs. Astro. del CIECEM | 06:34:25W 37:01:15N  | 35-cm      | QSI-516wsg        | C       | AIP4Win           |
| 11a  | Stará Lesná Obs.       | 20:17:25E 49:09:08N  | 60-cm      | FLI ML-3041       | C, Rc   | MaxIm-DL5         |
| 11b  | Stará Lesná Obs.       | 20:17:21E 49:09:06N  | 18-cm      | SBIG ST-10XME     | C       | MaxIm-DL5         |
| 12   | SAO RAS                | 41:26:26E 43:38:49N  | 1.0m       | EEV 42-40         | Rc      | MaxIm-DL5         |
| 13a  | Crimean Astropsy. Obs. | 34:00:57E 44:43:36N  | 1.25-m     | ProLine PL23042   | C,B,V,R | MAXIM DL          |
| 13b  | Crimean Astropsy. Obs. | 34:00:57E 44:43:36N  | 38-cm      | APOGEE ALTA E47   | C,B,V,R | MAXIM DL          |
| 13c  | Crimean Astropsy. Obs. | 34:00:57E 44:43:36N  | 2.6-m ZTSh | APOGEE ALTA E47   | BVR     | MAXIM DL          |
| 14   | Funao Astrono. Obs.    | 133:42:34E 34:34:55N | 28-cm      | Moravian G2-1600  | none    | AIP4Win           |
| 15   | Tokyo, Japan           | 130:41E 35:41N       | 30-cm      | SBIG ST-9XE       | C       | FitsPhot          |
| 16   | Nagasaki, Japan        | 129:53E 32:44N       | 35-cm      | SBIG ST10XME      | C,Rc    | FitsPhot          |
| 17   | Kyoto Univ.            | 135:46:59E 35:01:49N | 40-cm      | Apogee Alta U6    | C       |                   |
| 18   | Kamagaya, Japan        | 140:00E 35:46N       | 25-cm      | Apogee Alta F47   | C       | MaxImDL           |
| 19   | Budapest, Hungary      | 19:02E 47:30N        | 25-cm      | ALCCD5.2          | V,C     | IRAF              |
| 20   | Herefordshire,GB       | 02:39W 52:04N        | 35-cm      | SXV H9            | C,V     | AIP4WIN           |
| 21   | Kolonica, Slovakia     | 22:16E 48:56N        | 35-cm      | MII G2-1600       | C       | C-Munipack        |
| 22   | Astrolab Iris          | 02:54:45E 50:49:02N  | 68-cm      | STL 6303E         | V       | 3DLesvePhotometry |
| 23   | Switzerland            | 08:13E 46:49N        | 28-cm      | SBIG ST7XME       | C       | AIP4WIN           |
| 24   | New Mexico             | 105:31W 32:54N       | 35-cm      | SBIG ST10XME      | V       |                   |
| 25   | CBA Belgium Obs.       | 05:04E 50:45N        | 35-cm      | STT-3200ME        | C       | Peranso           |
| 26   | Sierra Remote Obs.     | 119:13W 37:20N       |            |                   | C       | VPhot             |
| 27   | AAVSO MT, US           |                      |            |                   | C       |                   |
| 28   | AFOEV FR               |                      |            |                   | C       |                   |
| 29   | AAVSO IL, US           |                      |            |                   | C       |                   |

\*Observers: 1 OKU Team, 2 NCU Team, 3 TSHAO Team, 4 A. Oksanen, 5 I. Miller, 6 S. Dvorak, 7 D. Starky, 8 S. Padovan, 9 NCU Team, 10 E. de Miguel, 11 SAS Team, 12 LMSU Team, 13 CrAO Team, 14 H. Akazawa/OUS Team, 15 H. Itoh, 16 Y. Maeda, 17 KU Team, 18 S. Kiyota, 19 T. Tordai, 20 R. Pickard, 21 P. A. Dubovsky, 22 F. Dubois Team, 23 K. Kasai, 24 V. Neustroev Team, 25 T. Vanmunster, 26 G. Stone, 27 R. Sabo, 28 E. Morelle., 29 J. Ulowetz

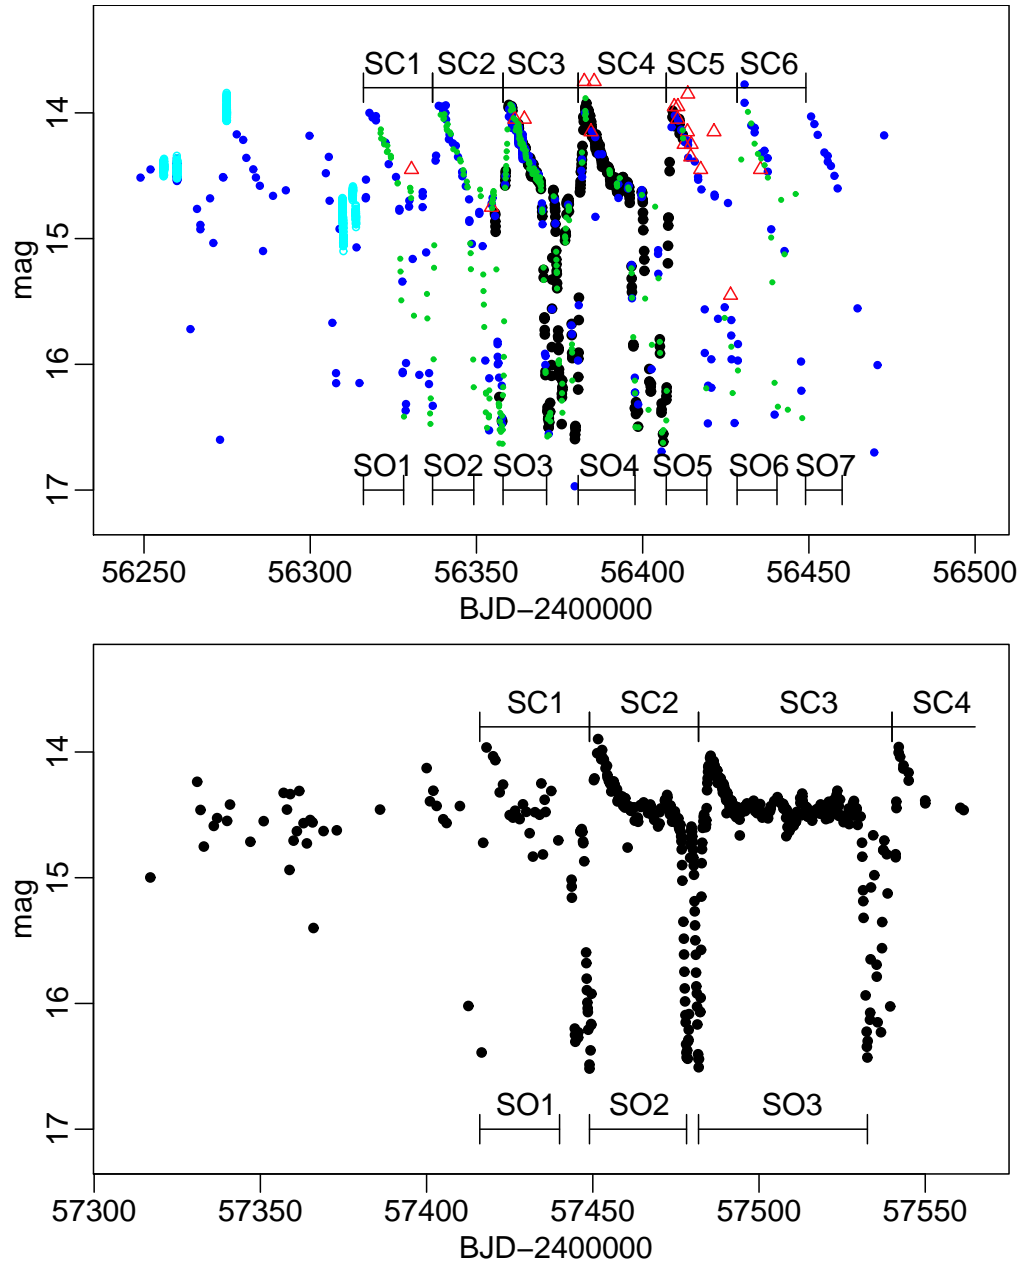

**E-figure 1.** Overall light curves of RZ LMi of 2013 (upper) and 2016 (lower) campaigns. In the upper panel, the black and green points indicate time-series unfiltered data binned to 0.1 d and V-band data from our observations. The blue and light blue points and red open squares indicate V-band, unfiltered CCD, and visual observations obtained from the AAVSO database.



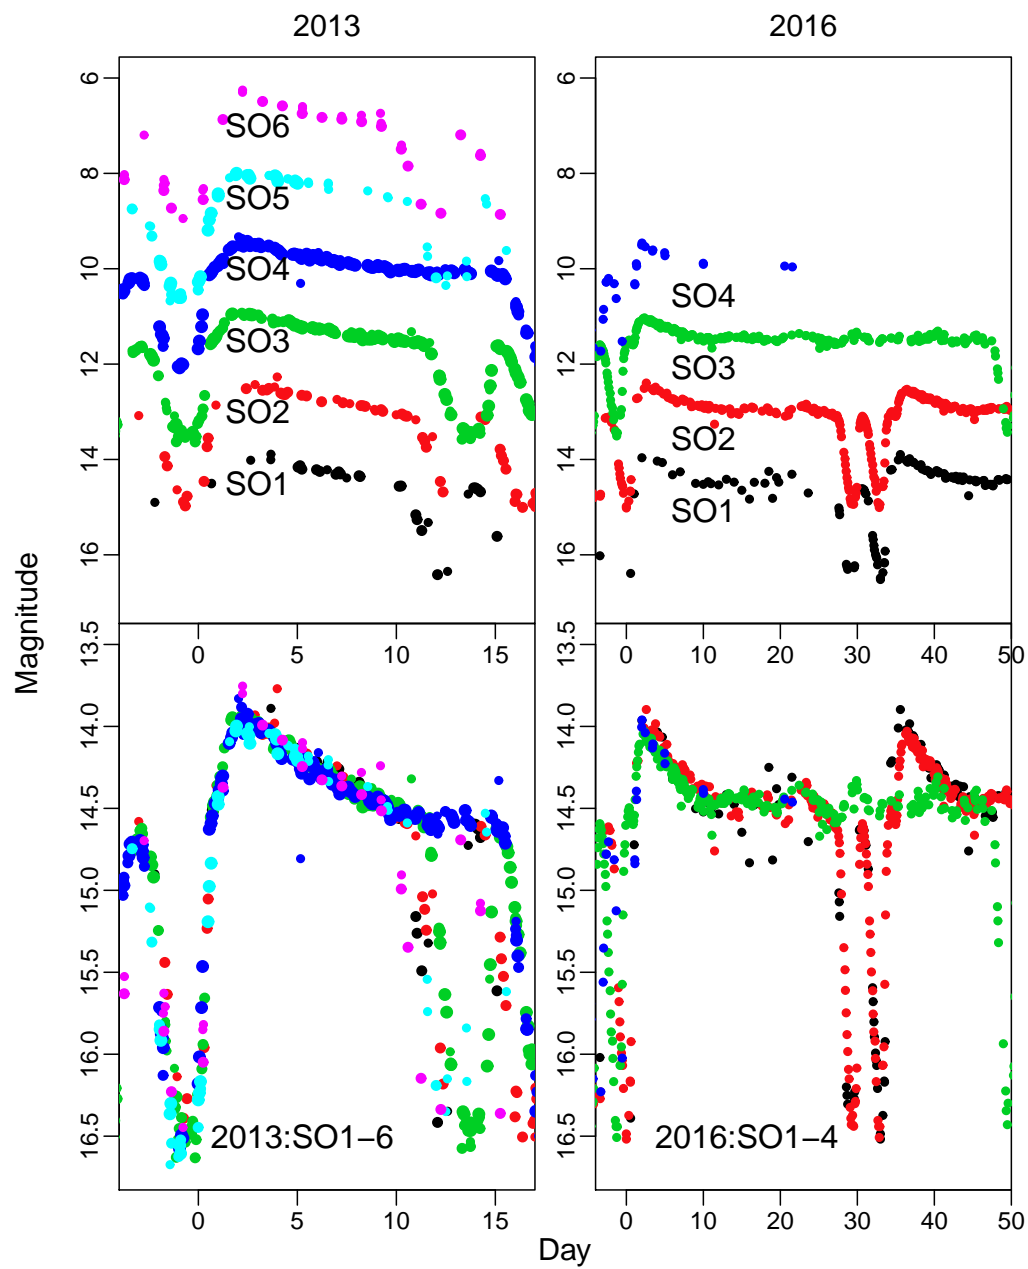

**E-figure 2.** Comparison of six superoutbursts in 2013 (Left) and four superoutbursts in 2016 (Right). The start of superoutbursts is set to be zero for each superoutburst.

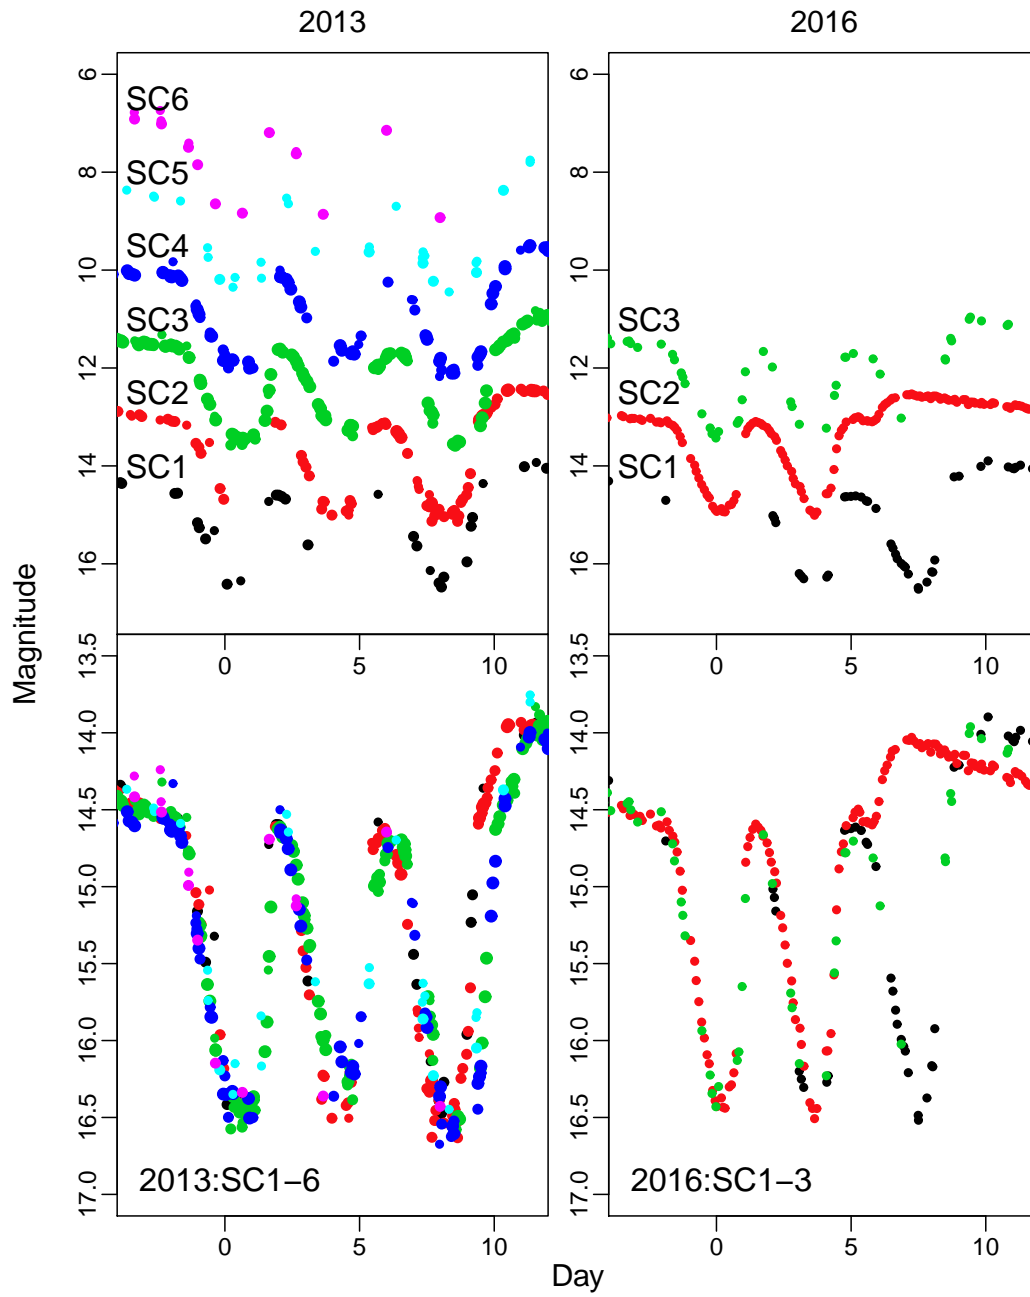

**E-figure 3.** Comparison of six non-superoutburst phases in 2013 (Left) and three non-superoutburst phases in 2016 (Right). The end of superoutbursts is set to be zero for each supercycle.



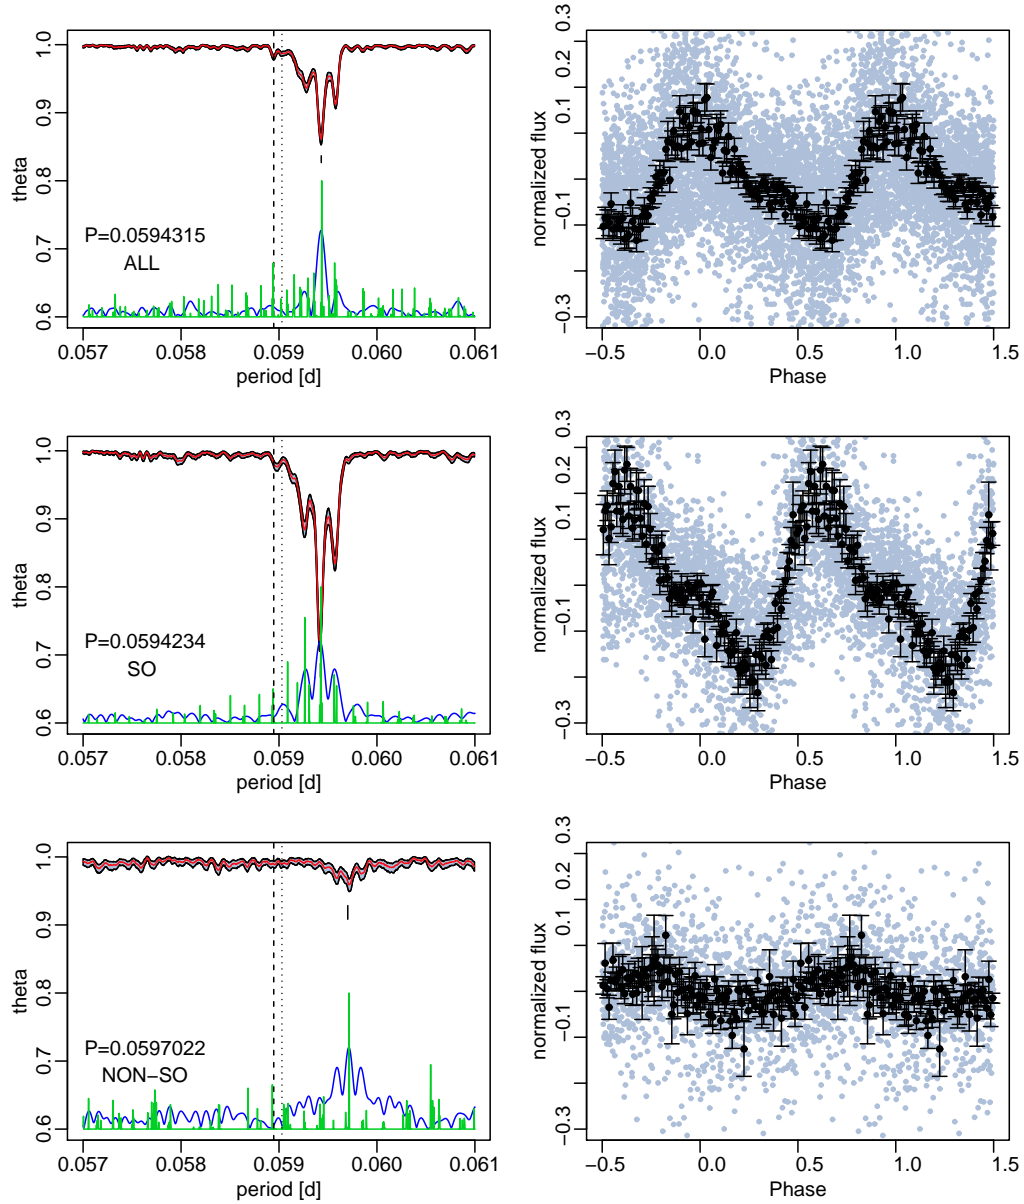

**E-figure 4.** Left: Period analysis of the whole time-series dataset in 2013 in pulsed flux scale. The red and green lines represent the results of the PDM and Lasso analysis, respectively. The blue lines at the bottom of the panels represent the window functions of the observations. The vertical dashed line shows a candidate of the orbital period (see the main text). The vertical dotted line shows an orbital period candidate detected by Kato et al. (2013). Right: Phase-averaged profiles folded by the superhump period.

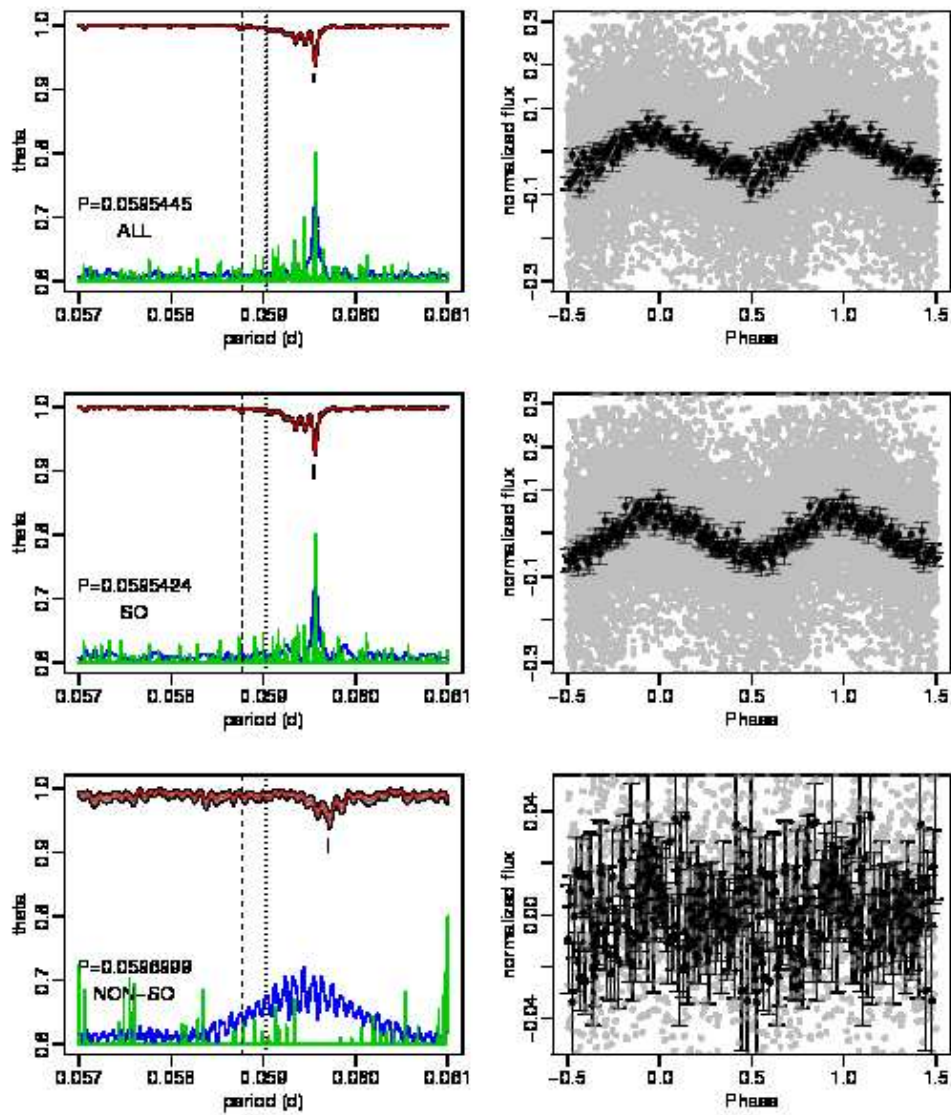

E-figure 5. The same with e-figure 4, but for the dataset in 2016.

**E-table 5.** Characteristics of Supercycles

| No.      | Start*<br>of SO | End*<br>of SO | NO1    | NO2   | End<br>of SC | Duration<br>of SO | Duration<br>of non-SO | Duration<br>of SC |
|----------|-----------------|---------------|--------|-------|--------------|-------------------|-----------------------|-------------------|
| 2013-SC1 | 16.1            | 28.1          | 30.2   | 33.7  | 36.8         | 12.0              | 8.7                   | 20.3              |
| 2013-SC2 | 36.8            | 49.2          | 51.0   | 54.8  | 58.0         | 12.4              | 8.5                   | 21.1              |
| 2013-SC3 | 58.0            | 71.1          | 73.1   | 77.4  | 80.6         | 13.4              | 9.5                   | 21.9              |
| 2013-SC4 | 80.6            | 97.7          | 99.7   | 103.8 | 107.1        | 17.1              | 9.4                   | 26.6              |
| 2013-SC5 | 107.1           | 119.3         | 121.4  | 125.6 | 128.4        | 12.2              | 9.1                   | 21.6              |
| 2013-SC6 | 128.4           | 140.4         | ~142.0 | 146.0 | >148.0       | 12.0              | >8                    |                   |
| 2016-SC1 | 17.1            | >40           | ~43    | 46.6  | 49.2         | >23               | <9                    | 32                |
| 2016-SC2 | 49.2            | 78.5          | 79.8   | 83.2  | 84.1         | 29.3              | 5.6                   | 34.9              |
| 2016-SC3 | 84.1            | 132.8         | 134.5  | 137.8 | 140          | 48.7              | 6.7                   | 56                |

\*BJD–2456300 for 2013 superoutbursts. BJD–2457400 for 2016 superoutbursts.

## E-section 5 $O - C$ Diagrams

We determined the times of superhump maxima by fitting using the template light curve as in Kato et al. (2009). As described in Kato et al. (2009), this usage of a fixed template (in this case, the best sampled superhump light curve of GW Lib) has an advantage of much higher signal-to-noise and thereby higher precision in determining maxima than eye estimates (typically reducing the scatter by a factor of  $\sim 5$ ) or than fitting using lower-quality template light curves prepared for individual objects. The usage of a fixed template, however, has a potential disadvantage of systematic errors caused by the variation in the superhump profile and the difference of the profile from the template. This effect has been confirmed to be negligible (cf. Kato et al. 2009) and we preferred higher precision. The potential effect of varying superhump profiles has been examined by comparison with a different method (PDM) and these methods have been confirmed to give consistent results (see e-section E-section 7). The resultant times are listed in e-tables 8–11.

E-figure 6 shows from the top to the bottom; 1. the general light curve, 2. the  $O - C$  diagram with the determined peak times and a linear ephemeris of  $\text{BJD}(\text{max}) = 2456359.73039 + 0.059422 \times E$  and, 3. the period determined from the  $O - C$  diagram, 4. two dimensional PDM period-theta diagram, and 5. two dimensional Lasso power spectrum, for the time series dataset in 2013. E-figure 7 is the same with e-figure 6 for 2016 data and the ephemeris used for the 2nd panel is  $\text{BJD}(\text{max}) = 2457452.569000 + 0.059503 \times E$ . Green and red points in the second panel of e-figure 6 represent the times of secondary peaks and those shifted by one cycle, respectively. The period from the  $O - C$  diagram was determined by a linear regression to the maxima within the window of 30 cycle counts ( $\sim 1.8$  d). The error refers to  $1\sigma$  error in the regression, and the errors of times of maxima are not taken into account. One should note that the period variation is smoothed by this method and the actual error should be larger than the errors shown. The

width of the moving window and the time step used for PDM and Lasso analysis are 1 d and 0.2 d, respectively.

The upper panel of e-figure 8 shows a comparison of the  $O - C$  diagrams for two superoutbursts in 2013 using ephemerides of  $\text{BJD}(\text{max}) = 2456358.54195 + 0.059422 \times E$  for the 3rd superoutburst and  $\text{BJD}(\text{max}) = 2456381.12202 + 0.059422 \times E$  for the 4th superoutburst. We set the cycle  $E = 20$  for the first maxima of fully grown superhumps in both superoutbursts. The two  $O - C$  diagrams are almost identical except for the longer plateau stage of the 4th superoutburst.

The lower panel of e-figure 8 shows a comparison of the  $O - C$  diagrams for two superoutbursts in 2016 using ephemerides of  $\text{BJD}(\text{max}) = 2457450.14798 + 0.0595596 \times E$  for the 2nd superoutburst and  $\text{BJD}(\text{max}) = 2457483.50085 + 0.0595596 \times E$  for the 3rd superoutburst. We set the cycle  $E = 20$  for the maxima at the superoutburst maximum (BJD 2454784.7052) in the 3rd superoutburst. The superoutburst maximum of the 2016-SO2 was not detected clearly, but it was around BJD 2454751.5. We set the cycle  $E = 40$  for the first maxima in the 2nd superoutburst. Again, the two  $O - C$  diagrams are consistent with each other except for the longer plateau stage of the 3rd superoutburst.

## E-section 6 Evolution of superhumps during superoutbursts

E-figures 9 and 10 show the evolution of the superhumps from the rising phase to the end of the superoutburst plateau during the 2013-SO3 (left) and 2013-SO4(right), and 2016-SO2 and 2016-SO3, respectively. Because the mean superhump periods obtained for the two superoutbursts in each year were very similar, we used an averaged period of 0.05945332 d for 2013, and 0.05954381 d for 2016 to fold nightly light curves and set the phase zero point to be BJD 2456360.5615, and 2456359.7304, respectively.

The amplitude of superhumps reached maximum around the

**E-table 6.** Superhump maxima of RZ LMi (2016 March)

| $E$ | max*       | error  | $O - C^\dagger$ | $N^\ddagger$ | $E$ | max*       | error  | $O - C^\dagger$ | $N^\ddagger$ |
|-----|------------|--------|-----------------|--------------|-----|------------|--------|-----------------|--------------|
| 0   | 57452.5390 | 0.0007 | 0.0065          | 49           | 201 | 57464.5014 | 0.0018 | 0.0007          | 47           |
| 1   | 57452.6016 | 0.0013 | 0.0095          | 33           | 215 | 57465.3295 | 0.0015 | -0.0048         | 112          |
| 29  | 57454.2612 | 0.0005 | 0.0019          | 26           | 216 | 57465.3975 | 0.0016 | 0.0037          | 121          |
| 31  | 57454.3783 | 0.0006 | -0.0001         | 33           | 217 | 57465.4504 | 0.0018 | -0.0030         | 128          |
| 32  | 57454.4414 | 0.0022 | 0.0034          | 17           | 249 | 57467.3529 | 0.0010 | -0.0058         | 58           |
| 42  | 57455.0297 | 0.0035 | -0.0036         | 30           | 250 | 57467.4147 | 0.0015 | -0.0035         | 61           |
| 43  | 57455.0919 | 0.0015 | -0.0010         | 46           | 251 | 57467.4722 | 0.0011 | -0.0056         | 57           |
| 44  | 57455.1510 | 0.0011 | -0.0014         | 65           | 267 | 57468.4339 | 0.0033 | 0.0034          | 61           |
| 45  | 57455.2096 | 0.0008 | -0.0024         | 66           | 268 | 57468.4948 | 0.0025 | 0.0048          | 63           |
| 46  | 57455.2698 | 0.0010 | -0.0017         | 37           | 322 | 57471.7050 | 0.0028 | -0.0004         | 29           |
| 47  | 57455.3279 | 0.0014 | -0.0032         | 22           | 323 | 57471.7688 | 0.0017 | 0.0039          | 29           |
| 51  | 57455.5659 | 0.0030 | -0.0033         | 57           | 324 | 57471.8282 | 0.0026 | 0.0038          | 31           |
| 63  | 57456.2832 | 0.0009 | -0.0005         | 45           | 325 | 57471.8851 | 0.0012 | 0.0010          | 33           |
| 65  | 57456.4001 | 0.0011 | -0.0027         | 77           | 328 | 57472.0794 | 0.0018 | 0.0167          | 100          |
| 68  | 57456.5826 | 0.0019 | 0.0011          | 35           | 329 | 57472.1215 | 0.0021 | -0.0007         | 153          |
| 80  | 57457.3048 | 0.0026 | 0.0088          | 32           | 333 | 57472.3616 | 0.0032 | 0.0013          | 76           |
| 81  | 57457.3507 | 0.0026 | -0.0048         | 36           | 334 | 57472.4158 | 0.0013 | -0.0041         | 45           |
| 83  | 57457.4705 | 0.0016 | -0.0041         | 33           | 335 | 57472.4780 | 0.0014 | -0.0015         | 42           |
| 84  | 57457.5370 | 0.0037 | 0.0029          | 69           | 336 | 57472.5394 | 0.0014 | 0.0004          | 40           |
| 99  | 57458.4225 | 0.0009 | -0.0048         | 62           | 345 | 57473.0716 | 0.0023 | -0.0033         | 161          |
| 100 | 57458.4864 | 0.0017 | -0.0005         | 80           | 346 | 57473.1356 | 0.0013 | 0.0012          | 164          |
| 102 | 57458.6050 | 0.0034 | -0.0009         | 66           | 351 | 57473.4286 | 0.0015 | -0.0036         | 86           |
| 110 | 57459.0806 | 0.0019 | -0.0016         | 55           | 352 | 57473.4892 | 0.0026 | -0.0025         | 106          |
| 111 | 57459.1435 | 0.0012 | 0.0017          | 61           | 361 | 57474.0269 | 0.0012 | -0.0007         | 134          |
| 150 | 57461.4719 | 0.0044 | 0.0079          | 88           | 362 | 57474.0850 | 0.0047 | -0.0021         | 161          |
| 151 | 57461.5198 | 0.0022 | -0.0037         | 39           | 363 | 57474.1457 | 0.0037 | -0.0010         | 158          |
| 165 | 57462.3587 | 0.0022 | 0.0016          | 62           | 372 | 57474.6858 | 0.0018 | 0.0033          | 26           |
| 181 | 57463.3040 | 0.0011 | -0.0058         | 49           | 373 | 57474.7455 | 0.0028 | 0.0034          | 32           |
| 197 | 57464.2664 | 0.0011 | 0.0039          | 81           | 384 | 57475.3990 | 0.0023 | 0.0019          | 51           |
| 198 | 57464.3208 | 0.0010 | -0.0013         | 116          | 385 | 57475.4517 | 0.0012 | -0.0049         | 42           |
| 199 | 57464.3810 | 0.0014 | -0.0006         | 111          | 395 | 57476.0521 | 0.0007 | 0.0000          | 102          |
| 200 | 57464.4380 | 0.0013 | -0.0031         | 103          | 396 | 57476.1117 | 0.0013 | 0.0002          | 290          |

\*BJD-2400000.

 $^\dagger$ Against max = 2457452.5325 + 0.059543*E*. $^\ddagger$ Number of points used to determine the maximum.

**E-table 7.** Superhump maxima of RZ LMi (2016 April)

| $E$ | max*       | error  | $O - C^\dagger$ | $N^\ddagger$ | $E$ | max*       | error  | $O - C^\dagger$ | $N^\ddagger$ |
|-----|------------|--------|-----------------|--------------|-----|------------|--------|-----------------|--------------|
| 0   | 57483.5067 | 0.0016 | -0.0041         | 64           | 71  | 57487.7335 | 0.0004 | -0.0021         | 53           |
| 5   | 57483.8081 | 0.0018 | -0.0002         | 32           | 72  | 57487.7930 | 0.0006 | -0.0021         | 50           |
| 8   | 57483.9877 | 0.0069 | 0.0009          | 138          | 76  | 57488.0300 | 0.0009 | -0.0032         | 112          |
| 9   | 57484.0522 | 0.0008 | 0.0058          | 250          | 77  | 57488.0886 | 0.0048 | -0.0040         | 33           |
| 10  | 57484.1065 | 0.0015 | 0.0006          | 283          | 78  | 57488.1482 | 0.0033 | -0.0040         | 25           |
| 12  | 57484.2236 | 0.0035 | -0.0013         | 79           | 82  | 57488.3934 | 0.0017 | 0.0033          | 138          |
| 13  | 57484.2944 | 0.0028 | 0.0101          | 63           | 83  | 57488.4472 | 0.0006 | -0.0024         | 185          |
| 14  | 57484.3515 | 0.0008 | 0.0076          | 273          | 84  | 57488.5031 | 0.0005 | -0.0061         | 157          |
| 15  | 57484.4110 | 0.0005 | 0.0077          | 305          | 93  | 57489.0406 | 0.0023 | -0.0041         | 93           |
| 16  | 57484.4694 | 0.0004 | 0.0065          | 234          | 98  | 57489.3387 | 0.0008 | -0.0035         | 84           |
| 17  | 57484.5284 | 0.0004 | 0.0060          | 241          | 99  | 57489.3994 | 0.0009 | -0.0023         | 62           |
| 18  | 57484.5873 | 0.0004 | 0.0054          | 55           | 100 | 57489.4557 | 0.0012 | -0.0055         | 36           |
| 19  | 57484.6525 | 0.0007 | 0.0112          | 24           | 104 | 57489.6951 | 0.0005 | -0.0042         | 51           |
| 20  | 57484.7052 | 0.0005 | 0.0043          | 42           | 106 | 57489.8142 | 0.0009 | -0.0041         | 50           |
| 22  | 57484.8249 | 0.0004 | 0.0050          | 82           | 106 | 57489.8140 | 0.0008 | -0.0042         | 47           |
| 29  | 57485.2404 | 0.0010 | 0.0039          | 48           | 109 | 57489.9883 | 0.0022 | -0.0085         | 132          |
| 30  | 57485.3019 | 0.0012 | 0.0060          | 73           | 110 | 57490.0534 | 0.0007 | -0.0029         | 276          |
| 31  | 57485.3628 | 0.0009 | 0.0073          | 144          | 111 | 57490.1116 | 0.0011 | -0.0042         | 241          |
| 32  | 57485.4176 | 0.0008 | 0.0027          | 134          | 112 | 57490.1667 | 0.0026 | -0.0086         | 99           |
| 33  | 57485.4767 | 0.0010 | 0.0023          | 118          | 115 | 57490.3482 | 0.0022 | -0.0056         | 95           |
| 34  | 57485.5367 | 0.0004 | 0.0028          | 143          | 116 | 57490.4097 | 0.0011 | -0.0036         | 119          |
| 35  | 57485.5937 | 0.0006 | 0.0003          | 63           | 117 | 57490.4679 | 0.0019 | -0.0049         | 51           |
| 36  | 57485.6566 | 0.0011 | 0.0036          | 55           | 119 | 57490.5882 | 0.0046 | -0.0037         | 39           |
| 37  | 57485.7110 | 0.0010 | -0.0015         | 83           | 120 | 57490.6490 | 0.0009 | -0.0023         | 122          |
| 38  | 57485.7759 | 0.0016 | 0.0039          | 85           | 121 | 57490.7062 | 0.0014 | -0.0046         | 65           |
| 39  | 57485.8333 | 0.0004 | 0.0018          | 46           | 122 | 57490.7672 | 0.0013 | -0.0031         | 52           |
| 42  | 57486.0144 | 0.0012 | 0.0044          | 19           | 123 | 57490.8216 | 0.0019 | -0.0082         | 52           |
| 43  | 57486.0696 | 0.0008 | 0.0001          | 22           | 133 | 57491.4224 | 0.0011 | -0.0025         | 60           |
| 44  | 57486.1277 | 0.0021 | -0.0013         | 17           | 136 | 57491.6013 | 0.0023 | -0.0021         | 90           |
| 45  | 57486.1907 | 0.0020 | 0.0022          | 21           | 137 | 57491.6580 | 0.0022 | -0.0049         | 91           |
| 46  | 57486.2558 | 0.0011 | 0.0078          | 52           | 138 | 57491.7160 | 0.0014 | -0.0064         | 80           |
| 47  | 57486.3081 | 0.0010 | 0.0006          | 73           | 150 | 57492.4317 | 0.0026 | -0.0048         | 74           |
| 48  | 57486.3643 | 0.0016 | -0.0027         | 70           | 151 | 57492.4926 | 0.0015 | -0.0033         | 30           |
| 49  | 57486.4270 | 0.0009 | 0.0005          | 144          | 153 | 57492.6113 | 0.0012 | -0.0037         | 68           |
| 50  | 57486.4826 | 0.0013 | -0.0034         | 162          | 154 | 57492.6717 | 0.0020 | -0.0028         | 67           |
| 53  | 57486.6660 | 0.0004 | 0.0015          | 87           | 159 | 57492.9777 | 0.0019 | 0.0057          | 21           |
| 54  | 57486.7222 | 0.0008 | -0.0018         | 103          | 160 | 57493.0284 | 0.0015 | -0.0031         | 138          |
| 55  | 57486.7839 | 0.0006 | 0.0004          | 134          | 161 | 57493.0825 | 0.0013 | -0.0085         | 148          |
| 56  | 57486.8406 | 0.0009 | -0.0025         | 63           | 169 | 57493.5658 | 0.0018 | -0.0012         | 87           |
| 59  | 57487.0207 | 0.0005 | -0.0009         | 281          | 170 | 57493.6251 | 0.0020 | -0.0014         | 89           |
| 60  | 57487.0799 | 0.0006 | -0.0012         | 279          | 171 | 57493.6804 | 0.0014 | -0.0056         | 80           |
| 61  | 57487.1329 | 0.0021 | -0.0077         | 117          | 172 | 57493.7409 | 0.0018 | -0.0046         | 34           |
| 65  | 57487.3794 | 0.0006 | 0.0009          | 72           | 173 | 57493.7999 | 0.0016 | -0.0052         | 33           |
| 66  | 57487.4376 | 0.0005 | -0.0005         | 67           | 177 | 57494.0384 | 0.0018 | -0.0047         | 151          |
| 68  | 57487.5554 | 0.0013 | -0.0017         | 60           | 178 | 57494.0957 | 0.0015 | -0.0069         | 244          |
| 68  | 57487.5543 | 0.0009 | -0.0028         | 60           | 187 | 57494.6349 | 0.0042 | -0.0032         | 91           |
| 69  | 57487.6242 | 0.0017 | 0.0076          | 26           | 198 | 57495.3070 | 0.0019 | 0.0143          | 32           |
| 70  | 57487.6769 | 0.0004 | 0.0008          | 50           | -   | -          | -      | -               | -            |

\*BJD-2400000.

 $^\dagger$ Against max = 2457483.5108 + 0.059504*E*. $^\ddagger$ Number of points used to determine the maximum.

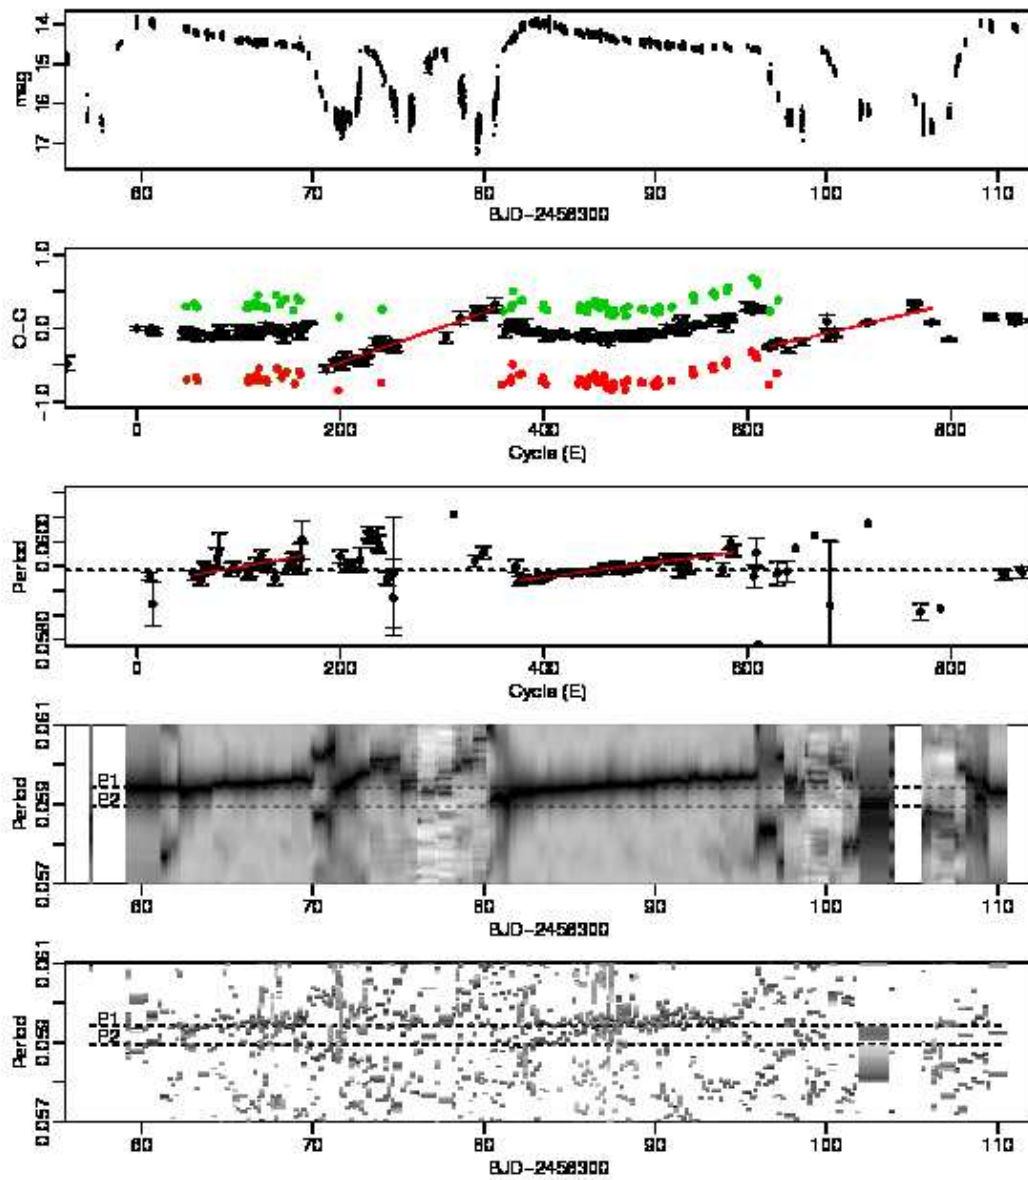

**E-figure 6.** Analysis of the 2013 observations. From top to the bottom: 1. general light curve, 2.  $O - C$  diagram, 3. period derived from the  $O - C$  diagram, 4. two dimensional PDM period- $\theta$  diagram, 5. two dimensional Lasso power spectrum



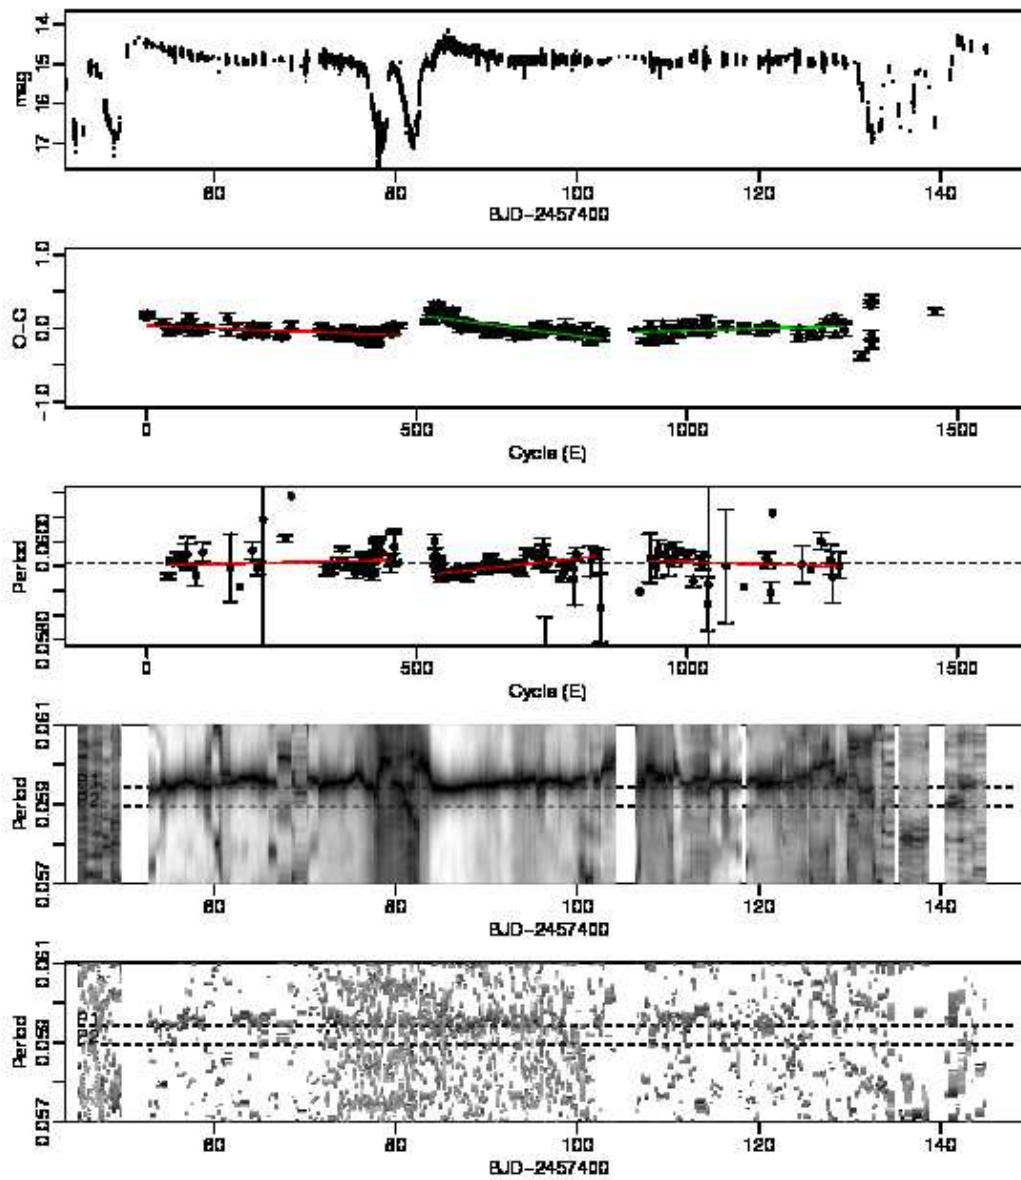

**E-figure 7.** Analysis of the 2016 observations. From top to the bottom: 1. general light curve, 2.  $O - C$  diagram, 3. period derived from the  $O - C$  diagram, 4. two dimensional PDM period- $\theta$  diagram, 5. two dimensional Lasso power spectrum



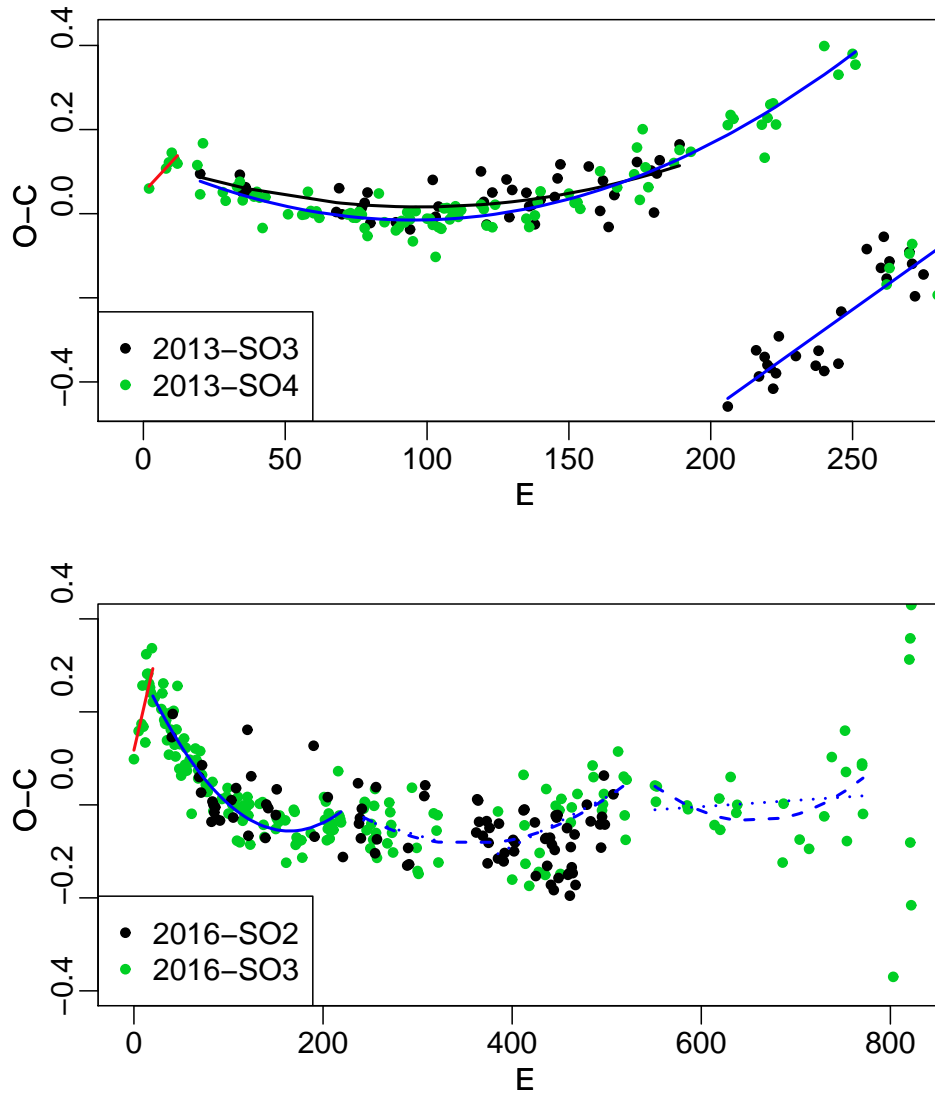

**E-figure 8.** Comparison of  $O - C$  curves between two superoutbursts in 2013 (upper) and 2016 (lower). Black and green points represent  $O - C$  values for respective superoutbursts. The cycle counts of the first maxima of fully grown superhumps are set to be 20 for both superoutbursts. Black and blue curves and dashed lines show the second order and linear fitting for  $O - C$  values during the stage B phases, respectively. Red lines are linear fitting for  $O - C$  values during the stage A phases.

**E-table 7.** Superhump maxima of RZ LMi (2016) (continued)

| $E$ | max*       | error  | $O - C^\dagger$ | $N^\ddagger$ | $E$ | max*       | error  | $O - C^\dagger$ | $N^\ddagger$ |
|-----|------------|--------|-----------------|--------------|-----|------------|--------|-----------------|--------------|
| 201 | 57495.4733 | 0.0034 | 0.0021          | 68           | 253 | 57498.5650 | 0.0043 | -0.0004         | 64           |
| 202 | 57495.5300 | 0.0025 | -0.0007         | 47           | 254 | 57498.6289 | 0.0024 | 0.0040          | 67           |
| 203 | 57495.5919 | 0.0018 | 0.0017          | 68           | 255 | 57498.6906 | 0.0057 | 0.0062          | 121          |
| 204 | 57495.6465 | 0.0019 | -0.0032         | 97           | 256 | 57498.7445 | 0.0016 | 0.0006          | 97           |
| 205 | 57495.7075 | 0.0012 | -0.0017         | 110          | 257 | 57498.8009 | 0.0014 | -0.0025         | 55           |
| 206 | 57495.7690 | 0.0021 | 0.0003          | 45           | 268 | 57499.4579 | 0.0022 | -0.0001         | 52           |
| 207 | 57495.8254 | 0.0021 | -0.0028         | 34           | 270 | 57499.5823 | 0.0016 | 0.0053          | 67           |
| 209 | 57495.9575 | 0.0044 | 0.0103          | 79           | 271 | 57499.6406 | 0.0022 | 0.0041          | 91           |
| 210 | 57496.0059 | 0.0011 | -0.0008         | 240          | 272 | 57499.6985 | 0.0013 | 0.0025          | 131          |
| 211 | 57496.0647 | 0.0031 | -0.0015         | 44           | 273 | 57499.7571 | 0.0014 | 0.0016          | 86           |
| 216 | 57496.3700 | 0.0019 | 0.0063          | 110          | 274 | 57499.8141 | 0.0033 | -0.0009         | 86           |
| 217 | 57496.4239 | 0.0010 | 0.0007          | 134          | 294 | 57501.0136 | 0.0023 | 0.0085          | 106          |
| 218 | 57496.4831 | 0.0017 | 0.0003          | 90           | 299 | 57501.3037 | 0.0024 | 0.0011          | 32           |
| 219 | 57496.5422 | 0.0022 | -0.0001         | 58           | 300 | 57501.3603 | 0.0026 | -0.0019         | 28           |
| 243 | 57497.9734 | 0.0014 | 0.0030          | 162          | 301 | 57501.4195 | 0.0040 | -0.0022         | 29           |
| 244 | 57498.0338 | 0.0008 | 0.0039          | 258          | 317 | 57502.3802 | 0.0012 | 0.0065          | 53           |
| 245 | 57498.0932 | 0.0008 | 0.0038          | 261          | 320 | 57502.5566 | 0.0028 | 0.0044          | 68           |
| 246 | 57498.1493 | 0.0011 | 0.0004          | 114          | 321 | 57502.6182 | 0.0014 | 0.0065          | 66           |
| 250 | 57498.3852 | 0.0017 | -0.0017         | 110          | 322 | 57502.6717 | 0.0024 | 0.0005          | 68           |
| 251 | 57498.4479 | 0.0016 | 0.0015          | 85           | —   | —          | —      | —               | —            |

\*BJD-2400000.

 $^\dagger$ Against max = 2457483.5108 + 0.059504*E*. $^\ddagger$ Number of points used to determine the maximum.

outburst maximum, and decreased for 6 d, then kept an almost constant value of  $\sim 0.1$  mag till the end of the plateau phase during both superoutbursts in 2013. The amplitude of superhumps during the two superoutbursts in 2016 shows a similar variation for about first 10 d, however, the amplitude increased again in the middle of the long plateau stage.

The profile of superhumps changed from the characteristic saw-tooth shape to doubly humped shape in the course of superoutbursts, though there was a hint of a secondary hump from the first day. The phases of these peaks gradually shifted toward smaller values for the first 5 d, then the direction changed toward larger values during both superoutbursts, confirming the changing superhump periods during the course of superoutbursts, as examined in e-section E-section 7.

### E-section 7 Variation of periods of superhumps during stage B

The mean periods derived from the  $O - C$  values of superhump maxima of stage B are 0.05944(1) d and 0.059496(7) d for 2013 SOs ( $20 \geq E \geq 189$  for 2013-SO3 and  $20 \geq E \geq 251$  for 2013-SO4 in the upper panel of e-figure 8), and 0.059544(3) d and 0.059552(2) d for 2016 SOs ( $40 \geq E \geq 507$  for 2016-SO2 and  $29 \geq E \geq 771$  for 2016-SO3 in the lower panel of e-figure 8).

The times of maxima in the longer plateau stages in 2016 superoutbursts affected the periods of 2016 SOs, since the later phase of such superoutbursts bear characteristics of standstills (or novalike state) rather than true superoutbursts as discussed in the main text. In order to make a comparison with the 2013 values, we used the peak times in early halves ( $E \geq 250$ ) of 2016 SOs. They gave mean periods of 0.05953(1) d and 0.059494(6) d, which are in good agreement with the values for 2013 SOs.

A positive period derivative ( $P_{\text{dot}} = \dot{P}/P$ ) which was suggested from observations of three superoutbursts in 2012 (Kato et al. 2013). The  $O - C$  values for our new observations gave a strong support for this positive  $P_{\text{dot}}$  as seen in e-figure 8. The times of superhump maxima in stage B in 2013 can be well expressed by the following equations:

$$\begin{aligned} \text{BJD}(\text{max}) \\ = 2456358.550(6) + 0.059216(59)E + 1.0(2) \times 10^{-6}E^2, \text{(E1)} \end{aligned}$$

and

$$\begin{aligned} \text{BJD}(\text{max}) \\ = 2456381.1274(8) + 0.059247(14)E \\ + 0.94(5) \times 10^{-6}E^2. \end{aligned} \quad \text{(E2)}$$

The lower panel of e-figure 8 indicates that the trend of the  $O -$

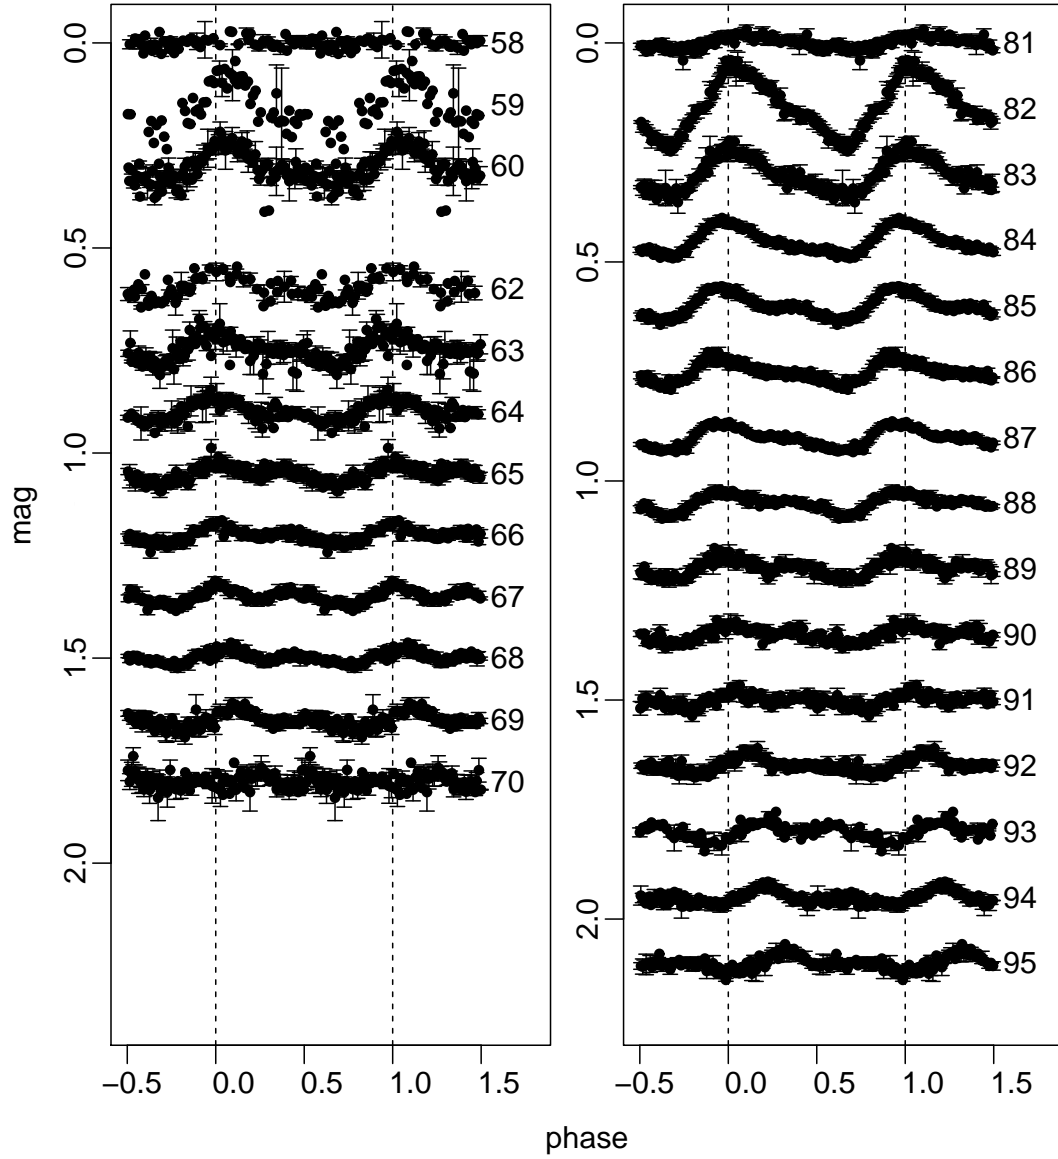

**E-figure 9.** Variation of superhump profiles during the 3rd superoutburst (left) and the 4th superoutburst (right) in 2013.

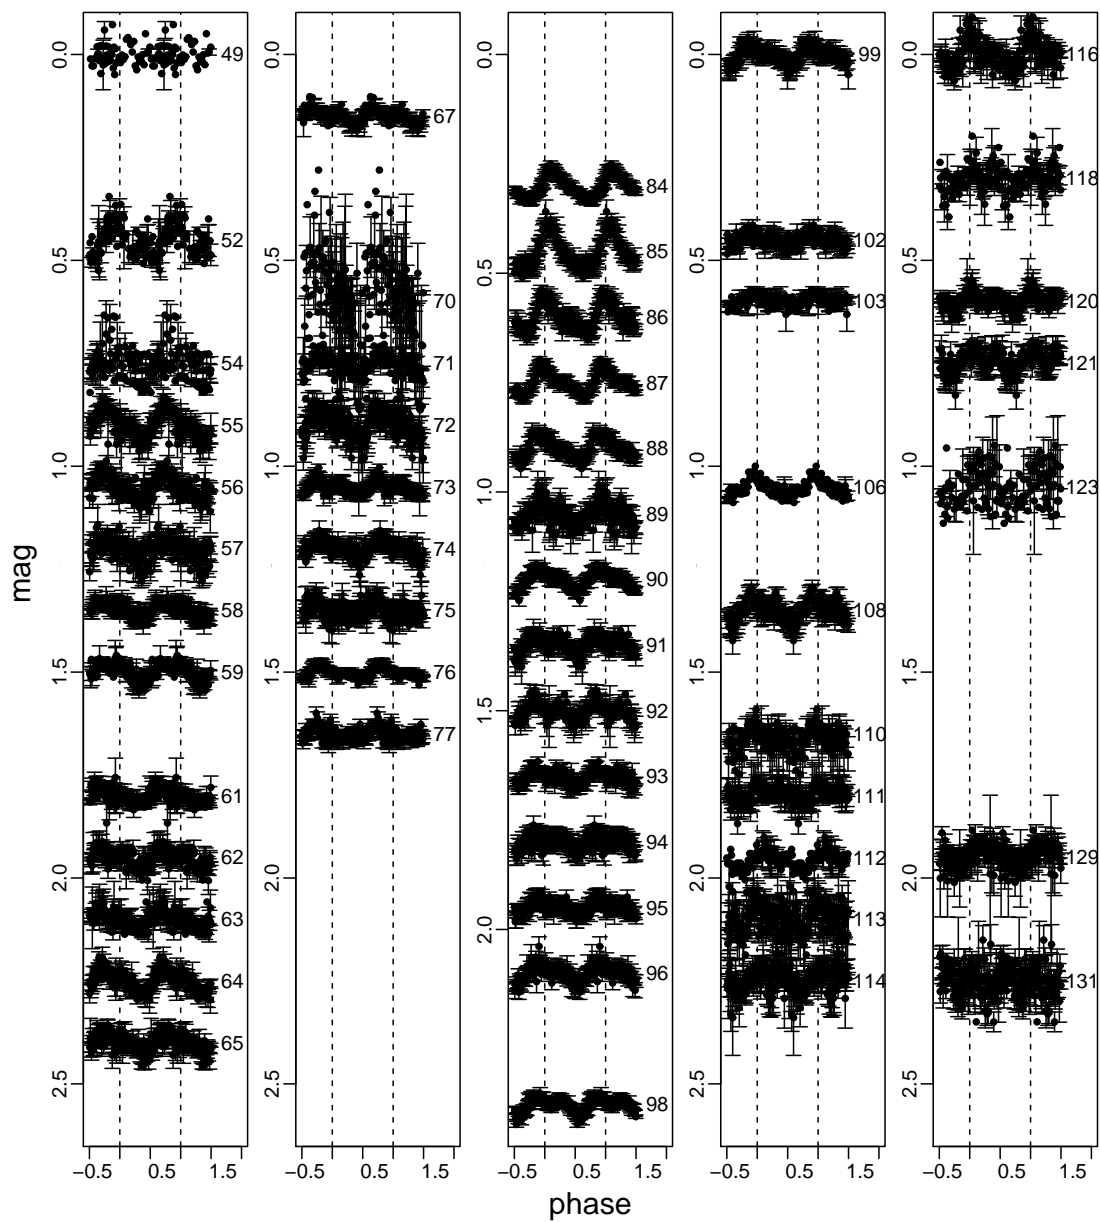

**E-figure 10.** Variation of superhump profiles during the 2nd superoutburst (1st and 2nd panels from the left) and the 3rd superoutburst (the other 3 panels) in 2016. We have omitted some nights only with low-quality data.

**E-table 8.** Superhump maxima of RZ LMi (2016 April, later part)

| $E$ | max*       | error  | $O - C^\dagger$ | $N^\ddagger$ | $E$ | max*       | error  | $O - C^\dagger$ | $N^\ddagger$ |
|-----|------------|--------|-----------------|--------------|-----|------------|--------|-----------------|--------------|
| 0   | 57506.4305 | 0.0008 | 0.0019          | 66           | 136 | 57514.5346 | 0.0063 | 0.0042          | 14           |
| 15  | 57507.3151 | 0.0018 | -0.0071         | 22           | 166 | 57516.3207 | 0.0028 | 0.0030          | 42           |
| 27  | 57508.0433 | 0.0023 | 0.0062          | 198          | 167 | 57516.3782 | 0.0012 | 0.0009          | 82           |
| 28  | 57508.0964 | 0.0018 | -0.0003         | 189          | 168 | 57516.4397 | 0.0027 | 0.0029          | 36           |
| 29  | 57508.1510 | 0.0054 | -0.0052         | 113          | 200 | 57518.3432 | 0.0040 | 0.0000          | 33           |
| 33  | 57508.3864 | 0.0018 | -0.0081         | 52           | 201 | 57518.4022 | 0.0013 | -0.0005         | 61           |
| 43  | 57508.9838 | 0.0021 | -0.0064         | 103          | 229 | 57520.0679 | 0.0016 | -0.0028         | 147          |
| 44  | 57509.0458 | 0.0026 | -0.0040         | 104          | 234 | 57520.3691 | 0.0015 | 0.0005          | 62           |
| 50  | 57509.4003 | 0.0017 | -0.0069         | 56           | 235 | 57520.4246 | 0.0030 | -0.0035         | 103          |
| 51  | 57509.4709 | 0.0046 | 0.0041          | 28           | 245 | 57521.0334 | 0.0065 | 0.0095          | 109          |
| 61  | 57510.0643 | 0.0018 | 0.0018          | 21           | 246 | 57521.0865 | 0.0012 | 0.0031          | 101          |
| 65  | 57510.3020 | 0.0012 | 0.0012          | 21           | 252 | 57521.4393 | 0.0011 | -0.0016         | 128          |
| 66  | 57510.3534 | 0.0030 | -0.0070         | 21           | 253 | 57521.4999 | 0.0027 | -0.0006         | 53           |
| 67  | 57510.4226 | 0.0025 | 0.0026          | 22           | 301 | 57524.3514 | 0.0028 | -0.0086         | 30           |
| 77  | 57511.0151 | 0.0033 | -0.0005         | 22           | 302 | 57524.4185 | 0.0014 | -0.0011         | 57           |
| 78  | 57511.0766 | 0.0070 | 0.0014          | 22           | 319 | 57525.4264 | 0.0033 | -0.0059         | 123          |
| 84  | 57511.4357 | 0.0014 | 0.0030          | 106          | 329 | 57526.0208 | 0.0025 | -0.0072         | 22           |
| 100 | 57512.3923 | 0.0028 | 0.0065          | 34           | 345 | 57526.9779 | 0.0048 | -0.0032         | 88           |
| 101 | 57512.4504 | 0.0014 | 0.0050          | 60           | 353 | 57527.4620 | 0.0015 | 0.0043          | 58           |
| 110 | 57512.9822 | 0.0030 | 0.0006          | 91           | 367 | 57528.2992 | 0.0018 | 0.0075          | 52           |
| 111 | 57513.0425 | 0.0062 | 0.0014          | 132          | 368 | 57528.3535 | 0.0022 | 0.0022          | 93           |
| 112 | 57513.1034 | 0.0017 | 0.0027          | 23           | 369 | 57528.4042 | 0.0020 | -0.0067         | 83           |
| 127 | 57514.0022 | 0.0039 | 0.0079          | 74           | 385 | 57529.3668 | 0.0015 | 0.0027          | 126          |
| 133 | 57514.3564 | 0.0008 | 0.0046          | 143          | 385 | 57529.3671 | 0.0015 | 0.0030          | 129          |
| 134 | 57514.4109 | 0.0007 | -0.0004         | 140          | 386 | 57529.4202 | 0.0049 | -0.0035         | 82           |
| 135 | 57514.4674 | 0.0015 | -0.0035         | 40           | —   | —          | —      | —               | —            |

\*BJD-2400000.

 $^\dagger$ Against max = 2457506.4286 + 0.059573*E*. $^\ddagger$ Number of points used to determine the maximum.

$C$  diagram changed several times during the long plateau stage in 2016: at around  $E=230$  and  $E=500$ . We cannot say whether there was a kink between  $E=322$  and 385 or  $O - C$  changed smoothly due to a 3.5 d-gap in the observation. The times of maxima in early parts of 2016 stage B ( $40 \geq E \geq 221$  for 2016-SO2 and  $20 \geq E \geq 219$  for 2016-SO3 in the lower panel of e-figure 8) can be well expressed by the following equations:

$$\text{BJD}(\text{max}) = 2457450.162(3) + 0.05937(6)E + 0.5(2) \times 10^{-6}E^2, \quad (\text{E3})$$

and

$$\text{BJD}(\text{max}) = 2457483.5199(9) + 0.05928(2)E + 0.83(7) \times 10^{-6}E^2. \quad (\text{E4})$$

The values of  $P_{\text{dot}}$  for stage B of each superoutburst are  $3.4(7) \times 10^{-5}$  for 2013-SO3,  $3.2(2) \times 10^{-5}$  for 2013-SO4,  $1.7(7) \times 10^{-5}$  for 2016-SO2, and  $2.8(2) \times 10^{-5}$  for 2016-SO2, which are in good agreement with each other within their re-

spective errors. These  $P_{\text{dot}}$  values are consistent with  $P_{\text{dot}}$  of  $2.4(1.5) - 4.9(3.6) \times 10^{-5}$  d in (Kato et al. 2013), though they are about a half of  $P_{\text{dot}} = 7.9(1.9) \times 10^{-5}$  in Olech et al. (2008).

E-figure 11 shows the results of the PDM analysis (left panels) and phase-averaged profiles (right panels) for the light curves during stage B of SO3 and SO4 in 2013. The mean superhump periods are calculated to be 0.059442(6) d and 0.059468(5) d, respectively, which are in good agreement with the mean periods of 0.05944(1) d and 0.059496(7) d by the  $O - C$  analysis. E-figures 12 and 13 show the same with e-figure 11 but for 2016 superoutbursts. The mean periods of whole plateau stages are 0.059552(2) d and 0.059537(2) d, and the periods for earlier halves of the plateau phase are 0.059532(6) d and 0.059493(3) d for two superoutbursts. The periods for earlier halves of the plateau phase are in good agreement with the mean periods of 0.05953(1) d and 0.059494(6) d by the  $O - C$  analysis.

These periods are in good agreement with the superhump

**E-table 9.** Superhump maxima of RZ LMi (2013)

| $E$ | max*       | error  | $O - C^\dagger$ | $N^\ddagger$ | $E$ | max*       | error  | $O - C^\dagger$ | $N^\ddagger$ |
|-----|------------|--------|-----------------|--------------|-----|------------|--------|-----------------|--------------|
| -69 | 57455.6076 | 0.0059 | -0.0227         | 50           | 197 | 57471.4135 | 0.0020 | -0.0230         | 57           |
| 0   | 57459.7360 | 0.0017 | 0.0056          | 30           | 199 | 57471.5351 | 0.0023 | -0.0202         | 59           |
| 14  | 57460.5678 | 0.0018 | 0.0055          | 38           | 200 | 57471.5934 | 0.0013 | -0.0214         | 114          |
| 15  | 57460.6247 | 0.0016 | 0.0030          | 62           | 201 | 57471.6524 | 0.0012 | -0.0218         | 124          |
| 16  | 57460.6849 | 0.0019 | 0.0037          | 54           | 202 | 57471.7089 | 0.0026 | -0.0247         | 147          |
| 17  | 57460.7435 | 0.0024 | 0.0029          | 46           | 203 | 57471.7705 | 0.0011 | -0.0225         | 222          |
| 48  | 57462.5829 | 0.0029 | 0.0002          | 21           | 204 | 57471.8351 | 0.0036 | -0.0173         | 45           |
| 49  | 57462.6457 | 0.0026 | 0.0036          | 21           | 210 | 57472.1889 | 0.0019 | -0.0201         | 39           |
| 50  | 57462.7014 | 0.0023 | -0.0001         | 20           | 217 | 57472.6035 | 0.0008 | -0.0215         | 54           |
| 57  | 57463.1183 | 0.0011 | 0.0008          | 33           | 218 | 57472.6650 | 0.0031 | -0.0194         | 125          |
| 58  | 57463.1784 | 0.0007 | 0.0015          | 33           | 220 | 57472.7810 | 0.0023 | -0.0222         | 46           |
| 59  | 57463.2393 | 0.0013 | 0.0030          | 32           | 225 | 57473.0791 | 0.0025 | -0.0212         | 43           |
| 60  | 57463.2944 | 0.0041 | -0.0013         | 20           | 226 | 57473.1459 | 0.0028 | -0.0138         | 43           |
| 69  | 57463.8293 | 0.0027 | -0.0012         | 39           | 235 | 57473.6896 | 0.0033 | -0.0050         | 103          |
| 74  | 57464.1254 | 0.0010 | -0.0022         | 38           | 240 | 57473.9840 | 0.0017 | -0.0077         | 46           |
| 82  | 57464.6078 | 0.0032 | 0.0048          | 37           | 241 | 57474.0478 | 0.0028 | -0.0033         | 58           |
| 83  | 57464.6620 | 0.0023 | -0.0004         | 43           | 242 | 57474.1013 | 0.0032 | -0.0092         | 56           |
| 84  | 57464.7228 | 0.0024 | 0.0010          | 26           | 243 | 57474.1632 | 0.0014 | -0.0067         | 85           |
| 99  | 57465.6191 | 0.0022 | 0.0060          | 99           | 250 | 57474.5805 | 0.0021 | -0.0054         | 59           |
| 100 | 57465.6743 | 0.0027 | 0.0017          | 94           | 251 | 57474.6382 | 0.0019 | -0.0071         | 53           |
| 101 | 57465.7305 | 0.0016 | -0.0015         | 107          | 252 | 57474.6931 | 0.0028 | -0.0117         | 54           |
| 103 | 57465.8538 | 0.0010 | 0.0030          | 43           | 255 | 57474.8744 | 0.0039 | -0.0086         | 29           |
| 108 | 57466.1528 | 0.0027 | 0.0048          | 39           | 304 | 57477.7928 | 0.0042 | -0.0018         | 38           |
| 109 | 57466.2069 | 0.0016 | -0.0005         | 38           | 318 | 57478.6405 | 0.0055 | 0.0139          | 43           |
| 110 | 57466.2702 | 0.0028 | 0.0034          | 39           | 334 | 57479.5941 | 0.0013 | 0.0168          | 59           |
| 115 | 57466.5669 | 0.0026 | 0.0030          | 49           | 335 | 57479.6556 | 0.0049 | 0.0188          | 59           |
| 116 | 57466.6244 | 0.0020 | 0.0010          | 91           | 336 | 57479.7149 | 0.0033 | 0.0187          | 51           |
| 117 | 57466.6840 | 0.0027 | 0.0012          | 83           | 337 | 57479.7708 | 0.0035 | 0.0152          | 57           |
| 118 | 57466.7407 | 0.0023 | -0.0015         | 60           | 351 | 57480.6086 | 0.0029 | 0.0211          | 46           |
| 120 | 57466.8630 | 0.0017 | 0.0020          | 117          | 352 | 57480.6722 | 0.0049 | 0.0253          | 47           |
| 125 | 57467.1605 | 0.0013 | 0.0024          | 163          | 362 | 57481.2444 | 0.0048 | 0.0033          | 32           |
| 126 | 57467.2225 | 0.0013 | 0.0050          | 109          | 368 | 57481.6038 | 0.0020 | 0.0061          | 69           |
| 127 | 57467.2840 | 0.0036 | 0.0070          | 43           | 369 | 57481.6641 | 0.0040 | 0.0070          | 90           |
| 137 | 57467.8779 | 0.0019 | 0.0067          | 62           | 370 | 57481.7248 | 0.0040 | 0.0083          | 58           |
| 141 | 57468.1093 | 0.0013 | 0.0004          | 78           | 371 | 57481.7833 | 0.0016 | 0.0074          | 86           |
| 142 | 57468.1730 | 0.0013 | 0.0047          | 97           | 372 | 57481.8422 | 0.0026 | 0.0068          | 64           |
| 144 | 57468.2853 | 0.0038 | -0.0019         | 67           | 379 | 57482.2579 | 0.0011 | 0.0066          | 55           |
| 146 | 57468.4086 | 0.0021 | 0.0026          | 130          | 380 | 57482.3132 | 0.0006 | 0.0024          | 76           |
| 154 | 57468.8887 | 0.0016 | 0.0073          | 76           | 381 | 57482.3798 | 0.0038 | 0.0097          | 47           |
| 159 | 57469.1846 | 0.0021 | 0.0061          | 72           | 388 | 57482.7889 | 0.0021 | 0.0027          | 19           |
| 160 | 57469.2381 | 0.0027 | 0.0002          | 45           | 389 | 57482.8471 | 0.0017 | 0.0015          | 21           |
| 161 | 57469.3030 | 0.0019 | 0.0057          | 56           | 393 | 57483.0868 | 0.0006 | 0.0035          | 48           |
| 162 | 57469.3643 | 0.0014 | 0.0075          | 60           | 394 | 57483.1469 | 0.0007 | 0.0042          | 48           |
| 169 | 57469.7825 | 0.0011 | 0.0098          | 73           | 395 | 57483.2037 | 0.0009 | 0.0016          | 47           |
| 186 | 57470.7556 | 0.0030 | -0.0272         | 36           | 399 | 57483.4419 | 0.0009 | 0.0021          | 61           |
| 196 | 57471.3578 | 0.0005 | -0.0193         | 58           | 400 | 57483.5020 | 0.0010 | 0.0028          | 55           |

\*BJD-2400000.

 $^\dagger$ Against max = 2456359.73039 + 0.059422*E*. $^\ddagger$ Number of points used to determine the maximum.

**E-table 10.** Superhump maxima of RZ LMi (2013) (continued)

| $E$ | max*       | error  | $O - C^\dagger$ | $N^\ddagger$ | $E$ | max*       | error  | $O - C^\dagger$ | $N^\ddagger$ |
|-----|------------|--------|-----------------|--------------|-----|------------|--------|-----------------|--------------|
| 401 | 57483.5606 | 0.0017 | 0.0020          | 37           | 484 | 57488.4916 | 0.0022 | 0.0010          | 56           |
| 402 | 57483.6157 | 0.0024 | -0.0023         | 26           | 495 | 57489.1433 | 0.0013 | -0.0010         | 69           |
| 403 | 57483.6795 | 0.0013 | 0.0020          | 35           | 496 | 57489.2015 | 0.0025 | -0.0022         | 82           |
| 411 | 57484.1525 | 0.0004 | -0.0004         | 38           | 498 | 57489.3220 | 0.0026 | -0.0005         | 89           |
| 416 | 57484.4495 | 0.0011 | -0.0004         | 62           | 499 | 57489.3833 | 0.0015 | 0.0013          | 142          |
| 417 | 57484.5090 | 0.0009 | -0.0004         | 64           | 500 | 57489.4442 | 0.0016 | 0.0029          | 87           |
| 418 | 57484.5716 | 0.0007 | 0.0028          | 130          | 510 | 57490.0382 | 0.0010 | 0.0025          | 56           |
| 419 | 57484.6283 | 0.0006 | 0.0001          | 104          | 512 | 57490.1557 | 0.0010 | 0.0012          | 104          |
| 420 | 57484.6874 | 0.0009 | -0.0002         | 102          | 513 | 57490.2152 | 0.0019 | 0.0013          | 100          |
| 421 | 57484.7471 | 0.0007 | 0.0000          | 87           | 514 | 57490.2737 | 0.0017 | 0.0004          | 70           |
| 422 | 57484.8056 | 0.0005 | -0.0009         | 52           | 521 | 57490.6949 | 0.0034 | 0.0057          | 44           |
| 432 | 57485.4003 | 0.0012 | -0.0004         | 83           | 527 | 57491.0492 | 0.0014 | 0.0034          | 62           |
| 433 | 57485.4599 | 0.0013 | -0.0002         | 74           | 533 | 57491.4076 | 0.0018 | 0.0053          | 41           |
| 434 | 57485.5187 | 0.0013 | -0.0009         | 61           | 534 | 57491.4708 | 0.0038 | 0.0091          | 41           |
| 435 | 57485.5781 | 0.0009 | -0.0009         | 104          | 535 | 57491.5228 | 0.0015 | 0.0017          | 46           |
| 436 | 57485.6383 | 0.0007 | -0.0000         | 58           | 536 | 57491.5922 | 0.0043 | 0.0116          | 45           |
| 437 | 57485.6974 | 0.0009 | -0.0004         | 56           | 537 | 57491.6463 | 0.0038 | 0.0063          | 75           |
| 438 | 57485.7549 | 0.0007 | -0.0023         | 59           | 538 | 57491.7029 | 0.0025 | 0.0034          | 85           |
| 439 | 57485.8132 | 0.0009 | -0.0034         | 57           | 547 | 57492.2411 | 0.0009 | 0.0069          | 77           |
| 443 | 57486.0569 | 0.0019 | 0.0026          | 34           | 549 | 57492.3618 | 0.0008 | 0.0087          | 79           |
| 445 | 57486.1717 | 0.0009 | -0.0015         | 43           | 553 | 57492.5992 | 0.0019 | 0.0085          | 45           |
| 449 | 57486.4082 | 0.0018 | -0.0027         | 46           | 566 | 57493.3755 | 0.0043 | 0.0122          | 34           |
| 450 | 57486.4680 | 0.0012 | -0.0023         | 62           | 567 | 57493.4363 | 0.0022 | 0.0136          | 36           |
| 451 | 57486.5284 | 0.0014 | -0.0013         | 62           | 568 | 57493.4952 | 0.0025 | 0.0131          | 36           |
| 452 | 57486.5876 | 0.0012 | -0.0015         | 88           | 578 | 57494.0886 | 0.0010 | 0.0123          | 47           |
| 453 | 57486.6485 | 0.0007 | -0.0001         | 58           | 579 | 57494.1433 | 0.0047 | 0.0076          | 36           |
| 454 | 57486.7069 | 0.0006 | -0.0011         | 53           | 580 | 57494.2084 | 0.0019 | 0.0132          | 61           |
| 455 | 57486.7632 | 0.0013 | -0.0042         | 91           | 581 | 57494.2697 | 0.0012 | 0.0151          | 71           |
| 456 | 57486.8269 | 0.0010 | 0.0001          | 116          | 582 | 57494.3293 | 0.0017 | 0.0153          | 47           |
| 460 | 57487.0635 | 0.0031 | -0.0010         | 31           | 583 | 57494.3857 | 0.0014 | 0.0123          | 54           |
| 461 | 57487.1229 | 0.0011 | -0.0010         | 75           | 600 | 57495.4070 | 0.0032 | 0.0234          | 45           |
| 462 | 57487.1815 | 0.0008 | -0.0019         | 59           | 605 | 57495.7000 | 0.0009 | 0.0193          | 77           |
| 463 | 57487.2364 | 0.0022 | -0.0064         | 47           | 610 | 57496.0001 | 0.0015 | 0.0223          | 63           |
| 464 | 57487.3000 | 0.0005 | -0.0022         | 60           | 611 | 57496.0580 | 0.0023 | 0.0208          | 62           |
| 465 | 57487.3592 | 0.0008 | -0.0024         | 100          | 622 | 57496.6806 | 0.0012 | -0.0103         | 67           |
| 466 | 57487.4215 | 0.0009 | 0.0005          | 142          | 623 | 57496.7423 | 0.0011 | -0.0080         | 78           |
| 467 | 57487.4810 | 0.0018 | 0.0005          | 62           | 630 | 57497.1603 | 0.0023 | -0.0059         | 31           |
| 468 | 57487.5388 | 0.0018 | -0.0011         | 62           | 631 | 57497.2211 | 0.0010 | -0.0046         | 30           |
| 469 | 57487.5988 | 0.0009 | -0.0005         | 77           | 640 | 57497.7487 | 0.0021 | -0.0118         | 37           |
| 470 | 57487.6595 | 0.0011 | 0.0008          | 57           | 654 | 57498.5868 | 0.0025 | -0.0056         | 31           |
| 471 | 57487.7174 | 0.0015 | -0.0007         | 56           | 678 | 57500.0297 | 0.0055 | 0.0112          | 42           |
| 472 | 57487.7778 | 0.0015 | 0.0002          | 39           | 680 | 57500.1366 | 0.0038 | -0.0007         | 42           |
| 479 | 57488.1945 | 0.0023 | 0.0010          | 55           | 686 | 57500.4964 | 0.0035 | 0.0025          | 44           |
| 480 | 57488.2533 | 0.0016 | 0.0004          | 62           | 718 | 57502.4052 | 0.0008 | 0.0098          | 58           |
| 481 | 57488.3104 | 0.0022 | -0.0020         | 60           | 719 | 57502.4656 | 0.0008 | 0.0108          | 57           |
| 483 | 57488.4290 | 0.0023 | -0.0022         | 51           | 764 | 57505.1551 | 0.0016 | 0.0263          | 48           |

\*BJD-2400000.

 $^\dagger$ Against max = 2456359.73039 + 0.059422*E*. $^\ddagger$ Number of points used to determine the maximum.



**E-table 11.** Superhump maxima of RZ LMi (2013) (continued)

| $E$ | max*       | error  | $O - C^\dagger$ | $N^\ddagger$ | $E$ | max*       | error  | $O - C^\dagger$ | $N^\ddagger$ |
|-----|------------|--------|-----------------|--------------|-----|------------|--------|-----------------|--------------|
| 765 | 57505.2107 | 0.0025 | 0.0225          | 36           | 862 | 57510.9678 | 0.0014 | 0.0156          | 41           |
| 781 | 57506.1493 | 0.0011 | 0.0103          | 54           | 863 | 57511.0220 | 0.0016 | 0.0104          | 48           |
| 798 | 57507.1460 | 0.0012 | -0.0031         | 54           | 864 | 57511.0828 | 0.0013 | 0.0118          | 47           |
| 839 | 57509.6008 | 0.0016 | 0.0154          | 55           | 880 | 57512.0347 | 0.0005 | 0.0129          | 54           |
| 840 | 57509.6592 | 0.0018 | 0.0143          | 55           | 881 | 57512.0923 | 0.0003 | 0.0111          | 54           |

\*BJD-2400000.

 $^\dagger$ Against max = 2456359.73039 + 0.059422 $E$ . $^\ddagger$ Number of points used to determine the maximum.

periods obtained for each of six outbursts by Olech et al. (2008). They are, however, slightly longer than the period of 0.05940 d obtained by (Olech et al. 2008) from a combined data of three superoutbursts and much shorter than the period of 0.059585(1) d obtained by Kato et al. (2013) from another three consecutive superoutbursts. As is evident from our new observations, superhump periods indeed vary during superoutbursts and superhump are not coherent in phases between different superoutbursts, a combined analysis of different superoutbursts is not adequate for determining superhump periods.

The superhump periods at the beginning and end of stage B calculated from the equations E1 and E2 are 0.05929 d and 0.059569 d for 2013-SO3, and 0.05929 d and 0.059758 d for 2013-SO4, respectively.

## References

- Fernie, J. D. 1989, PASP, 101, 225  
Kato, T., et al. 2013, PASJ, 65, 23  
Kato, T., et al. 2009, PASJ, 61, S395  
Kato, T., et al. 2010, PASJ, 62, 1525  
Kato, T., & Uemura, M. 2012, PASJ, 64, 122  
Olech, A., Wisniewski, M., Zloczewski, K., Cook, L. M., Mularczyk, K., & Kedzierski, P. 2008, Acta Astron., 58, 131  
Osaki, Y., & Kato, T. 2013a, PASJ, 65, 50  
Osaki, Y., & Kato, T. 2013b, PASJ, 65, 95  
Osaki, Y., & Meyer, F. 2003, A&A, 401, 325  
Stellingwerf, R. F. 1978, ApJ, 224, 953

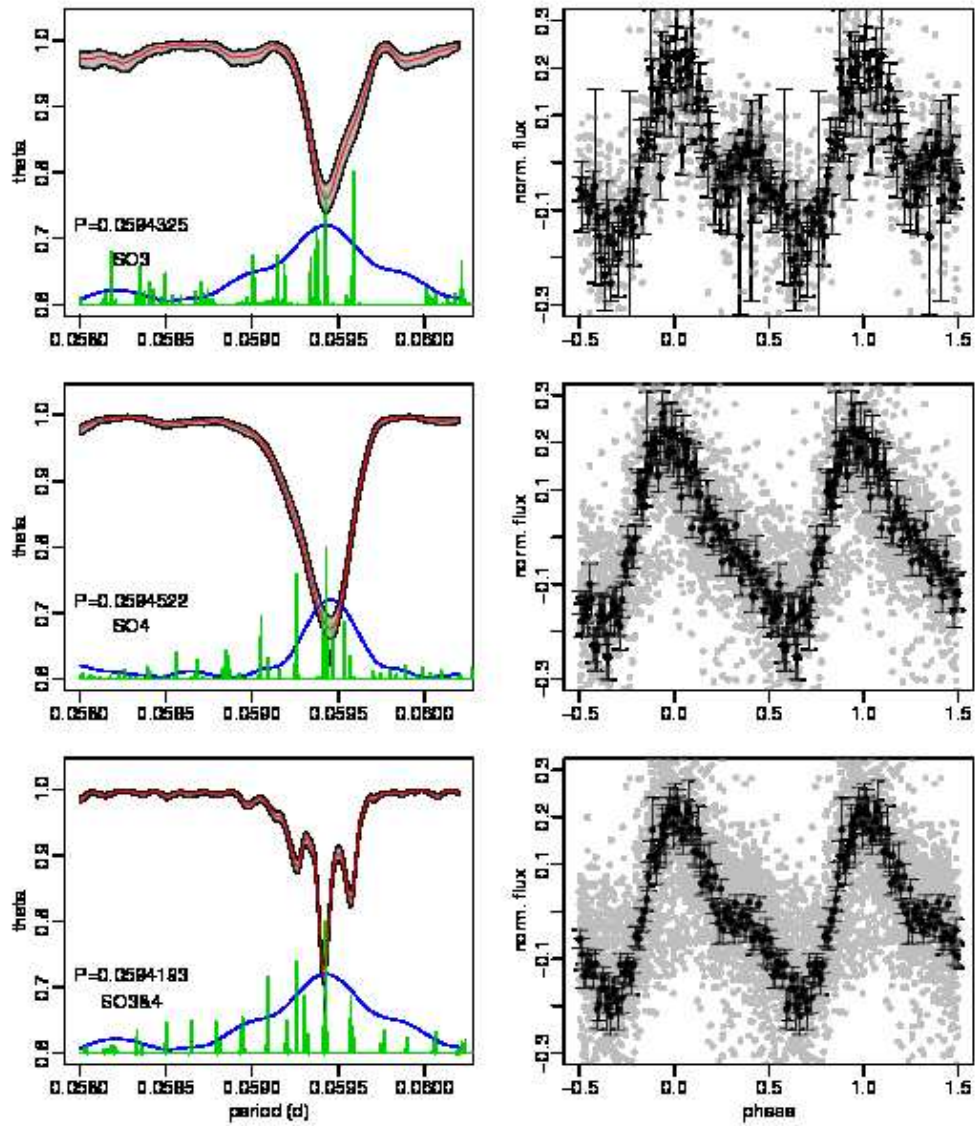

**E-figure 11.** Left panels show period analysis of plateau phases, and right panels show phase-averaged superhump profiles of the 3rd superoutburst (upper) and the 4th superoutburst (lower) in 2013.

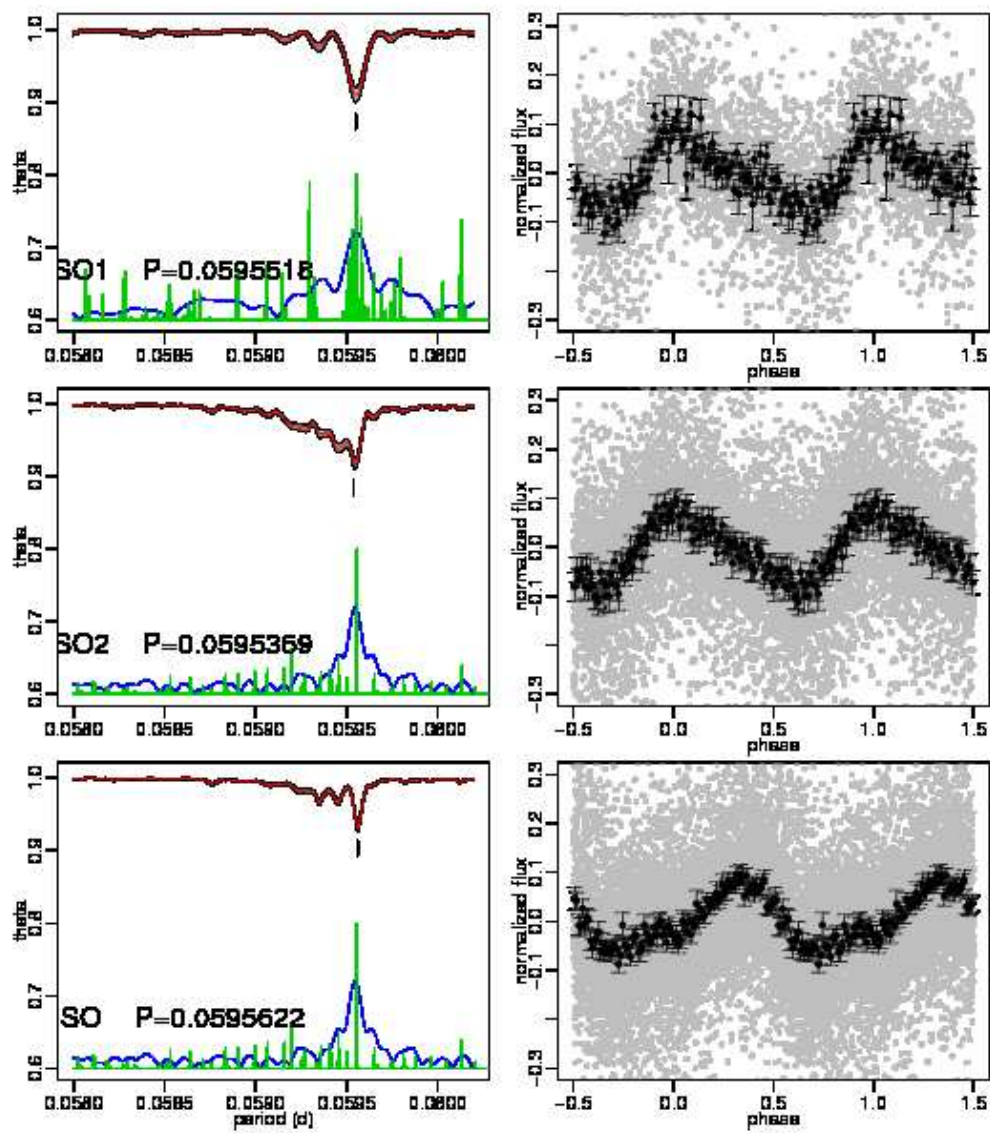

E-figure 12. The same as e-figure 11, but of the 2nd (upper) and 3rd (lower) superoutbursts in 2016.

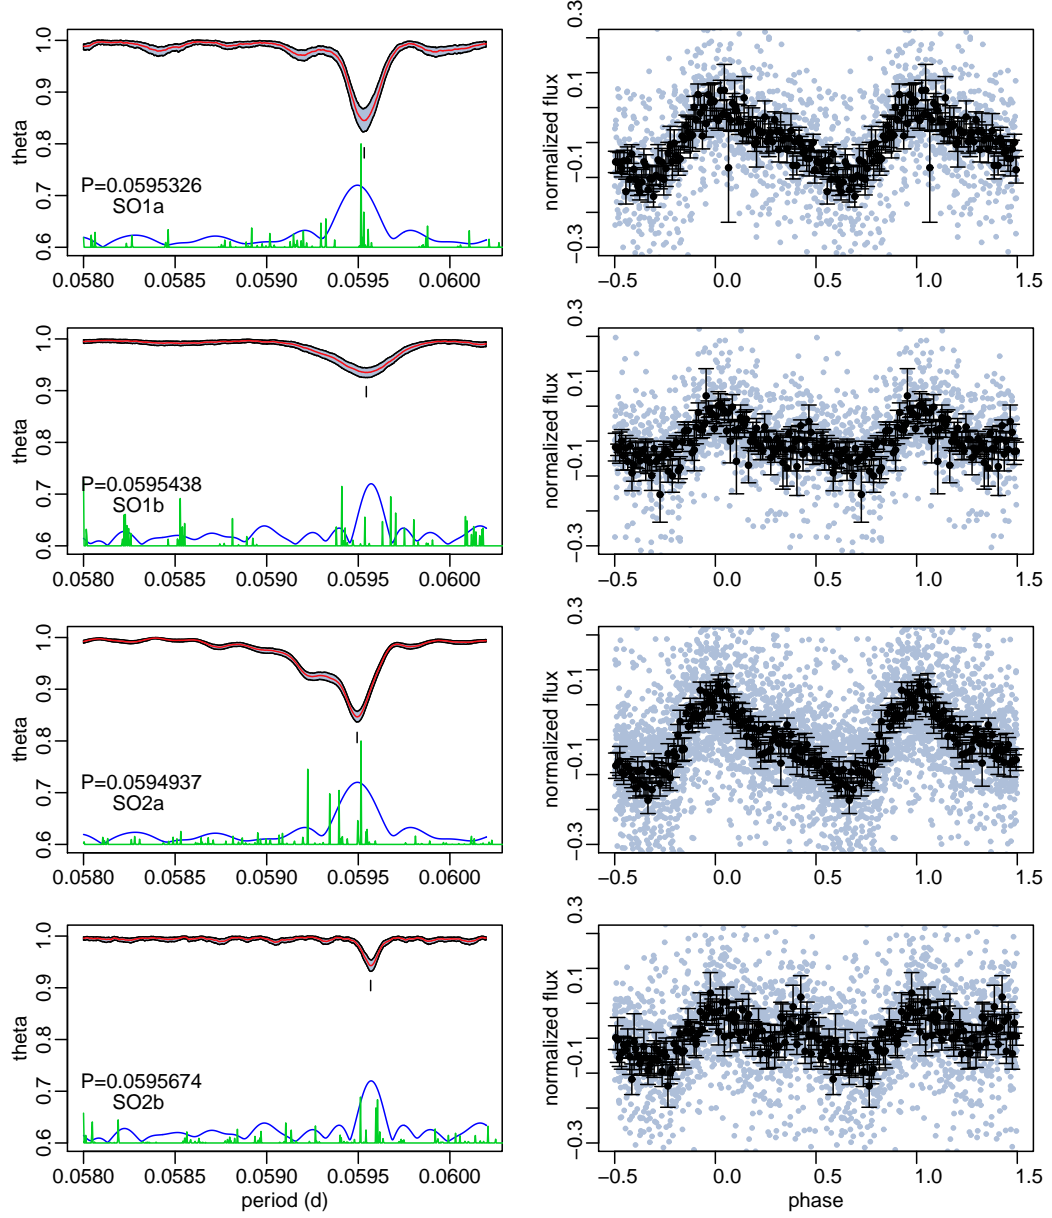

**E-figure 13.** The same as e-figure 12, but of the data between BJD 2457449 and 2457470, BJD 2457470 and 2457478.5, BJD 2457484 and 2457503, and BJD 2457503 and 2457535 were used (from the top to the bottom).
